# Supplementary material for: CAPTURE: Minimizing Watch Time for Reliable Temporal Video Grounding
Source: arXiv:2611.38466 source file (2026-11-28)
Supplement: Supplementary file 1 [file qualitative-failure.tex]

\begin{figure}[tbp]
\centering
\includegraphics[width=\columnwidth]{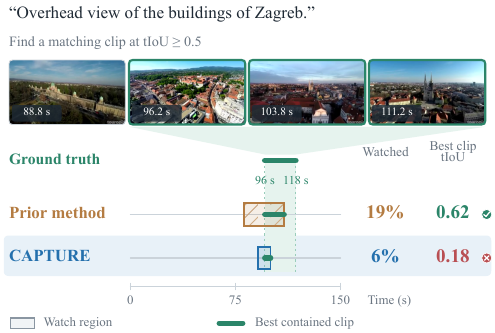}
\caption{\textbf{Reaching part of the moment is not always enough.}
\texttt{CAPTURE}'s region starts too early and contains only 4 of the annotated moment's 22 seconds.
Its best clip tIoU is 0.18, below the requested 0.5.
The prior method reaches 0.62 while watching more.
Marginal coverage does not ensure success on every query.}
\label{fig:supp:qualitative-failure}
\end{figure}
