# Supplementary material for: CAPTURE: Minimizing Watch Time for Reliable Temporal Video Grounding
Source: arXiv:2611.38466 source file (2026-11-28)
Supplement: Supplementary file 2 [file qualitative-success.tex]

\begin{figure}[tbp]
\centering
\includegraphics[width=\columnwidth]{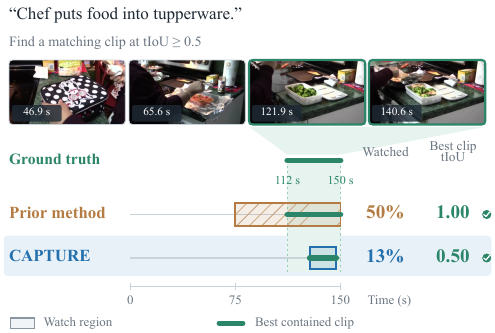}
\caption{\textbf{A matching clip can require much less viewing than the whole moment.}
\texttt{CAPTURE} returns 19 of the moment's 38 seconds, reaching tIoU 0.5 while watching 13\% of the video.
The prior method watches 50\%.
Green outlines mark frames inside the annotated moment.
Best clip tIoU is the highest tIoU of any clip within the returned footage.}
\label{fig:supp:qualitative-success}
\end{figure}
