# Supplementary material for: CAPTURE: Minimizing Watch Time for Reliable Temporal Video Grounding
Source: arXiv:2611.38466 source file (2026-11-28)
Supplement: Supplementary file 3 [file twoprompt.tex]

\begin{figure*}[t]
\centering
\includegraphics[width=\textwidth]{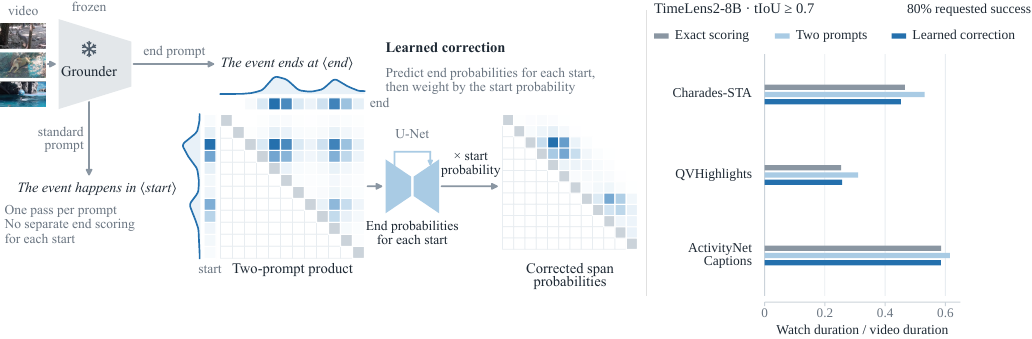}
\caption{\textbf{A learned correction reduces the extra viewing from two-prompt scoring.}
On the left, two prompts score starts and ends independently.
A U-Net predicts end probabilities conditional on each start, then multiplies by the start probability to form corrected span probabilities without further grounder passes.
On the right, the exact anchor with continuation uses TimeLens2-8B at tIoU 0.7 and 80\% requested success over 1,000 trials.
On QVHighlights, the correction lowers watch duration from 31\% to 26\% of the video, close to 25\% with exact scoring.}
\label{fig:supp:twoprompt}
\end{figure*}
