# Supplementary material for: CAPTURE: Minimizing Watch Time for Reliable Temporal Video Grounding
Source: arXiv:2611.38466 source file (2026-11-28)
Supplement: Supplementary file 4 [file implementation.tex]

\section{\texttt{CAPTURE} implementation}
\label{sec:supp:impl}

\texttt{CAPTURE} scores candidate spans, orders them to form nested watched regions, and calibrates where to stop.
We use fit videos to choose $q_0$ and, for supplementary variants, the region type.
Independent calibration videos then determine the final threshold.
Throughout the experiments, success means that the returned region contains a matching clip.

\subsection{Exact span probabilities}
\label{sec:supp:impl:scoring}
\label{sec:capture:score}

\paragraph{Scoring all spans.}
We compute $Q(y\mid X)=p_f(y\mid X)$ for every whole-second candidate span.
The model encodes the video once.
Starting from a fixed answer prefix, a token tree scores every possible start time.
A tree branching from each start then scores every later end time.
Span scores include start, separator, end and closing-token probabilities.
Caching the video--query representation preserves sequential-decoding scores up to bfloat16 rounding.
MiMo-VL-7B assigns more start-time probability to whole seconds in angle brackets than to minutes and seconds, so we use that format.
Separate greedy decoding supplies the baselines' single answer.

\paragraph{Retained probability and timestamp resolution.}
We keep the 12,000 most probable spans per query and renormalize their probabilities to sum to 1.
Calibration and test videos on the three main benchmarks last at most 150.02 seconds. Their complete whole-second pools contain fewer than 12,000 spans, so the cap removes none.
The whole-second pool can still omit some model probability.
Before renormalization, its median total probability is 0.998 to 0.9999 for TimeLens~\cite{zhang2025timelens,zhu2026timelens2}, 0.04 to 0.10 for Qwen3-VL~\cite{bai2025qwen3vl} and 0.15 to 0.25 for MiMo-VL-7B~\cite{xiaomi2025mimovl}.
The remaining probability goes to other timestamp resolutions or formats, including tenths of seconds for Qwen3-VL and minutes and seconds for MiMo-VL-7B.

Marginal coverage under the region rule does not depend on the total probability before renormalization.
A calibration query receives score 1 if no prefix of the retained pool succeeds.
If calibration selects $\hat q=1$, prediction returns all candidate subclips from the entire video, bypassing the retained pool (\cref{thm:validity}).

On QVHighlights, summing probabilities over timestamps written in tenths of a second raises Qwen3-VL's median retained probability to 0.99.
Each end-time variant is scored with its start written as, for example, \texttt{12.0} instead of \texttt{12}.
Across the six requests, normalized watch duration with the exact anchor changes by $-0.024$ to $-0.007$ for Qwen3-VL-4B and $-0.019$ to $+0.009$ for Qwen3-VL-8B.

\paragraph{Computation time.}
\Cref{tab:supp:runtime} separates decoding, generation and scoring time on an idle H200 GPU.
TimeLens2-8B uses about 30\,GiB, including weights.
Region construction and continuation take a median 0.08 seconds once probabilities are available.
These times exclude calibration, which runs once before testing.
\supptab{set_runtime}

\subsection{Approximate span probabilities}
\label{sec:supp:impl:factorized}

\paragraph{Scoring starts and ends separately.}
When exact joint scoring is unavailable or expensive, two prompts provide separate start and end probabilities.
This avoids end scoring separately for every start.
The end prompt asks ``Please find the visual event described by the sentence `$\{Q\}$', determining its ending time. The format should be: `The event ends at $\langle$end time$\rangle$ seconds'.'' %
Here $\{Q\}$ is the text query.
With the cached video representation, one pass after ``The event ends at'' gives the whole-second end distribution $\bar p_f(e\mid X)$.
The original temporal-grounding prompt gives the whole-second start distribution $\bar p_f(s\mid X)$.
For $s<e$, we form the two-prompt product $\tilde p_f([s,e]\mid X)\propto\bar p_f(s\mid X)\,\bar p_f(e\mid X)$ and renormalize over the scored spans as for exact joint scoring.

\paragraph{Learning the dependence between endpoints.}
The two-prompt product treats start and end times independently.
The learned correction instead predicts the end distribution conditional on each start.
Multiplying by the start distribution approximates their joint distribution.
For each candidate start, the network receives the full start distribution and the end-prompt probabilities for all later ends.
Additional channels at each start--end grid cell encode span validity, position, duration and bin size.
A U-Net processes the grid, with row and column attention at its two coarsest levels (\cref{fig:supp:twoprompt}).

We divide each target benchmark's fit videos into four folds.
Each of four networks trains on three folds and all queries from the other two benchmarks.
Each target fit video is evaluated by the network that excluded its fold.
For calibration and testing, we average predictions from all four networks.
None trains on any target calibration or test query.

This avoids another grounder pass per start.
We measure total-variation distance between predicted and exact conditional end distributions, averaging with start weights $\bar p_f(s\mid X)$.
\Cref{sec:exp:structure} reports accuracy and watch duration.

\paragraph{Correction for longer videos.}
Charades-STA-Long uses a correction trained on its own fit videos and the main benchmarks, excluding calibration and test sources (\cref{sec:supp:results:long}).
Exact scoring remains the reference when feasible.

\input{fig/supp/twoprompt}

\subsection{Region construction and calibration}
\label{sec:supp:impl:regions}

\paragraph{Main-paper exact-anchor configuration.}
\label{sec:supp:watch}
When all whole-second spans are retained, \cref{alg:s:capture} converts the shortest region from \cref{alg:watch} into an inclusion-minimal anchor.
The ordering $\pi_X=\operatorname{Order}(X,A(X))$ places its spans first, followed by all remaining spans, with each group sorted by decreasing model probability.
The main paper calibrates this order directly (\cref{alg:capture_calibration,alg:capture_prediction}), without the continuation described below.
We use fit videos to choose $q_0\in\{0.6,0.7,0.8,0.9,0.95,0.98,0.99,0.995\}$.
\emph{Segments} counts separate watched intervals on the whole-second grid.

On long videos where we cap the pool, we construct the anchor using the renormalized retained probabilities.
The dynamic program may find a region containing a matching clip that is absent from the retained pool.
Its region success probability can then reach $q_0$ while the retained spans inside it still have span-set success probability below $q_0$.
We increase the watch-duration budget until those spans reach $q_0$.
This anchor meets the threshold but need not minimize watch duration over retained spans, so \cref{thm:watch} need not apply.
At threshold 1, prediction bypasses the cap and returns the entire video, preserving marginal coverage.

\paragraph{Exact anchor with continuation.}
This variant reorders up to 40 spans after the anchor, keeping the anchor and calibration rule.
It first adds remaining spans inside the watched region at no extra watch time.
Otherwise, it adds the span with the largest model-estimated success gain per newly watched second.
The rest follow in decreasing probability.

\paragraph{Alternative anchors and orders.}
The gain-per-second anchor uses this selection rule starting from an empty region.
It first adds spans that cost no extra watch time, then chooses the largest success gain per newly watched second.
It stops when model-estimated success strictly exceeds $q_0$ and removes any span whose deletion leaves success strictly above $q_0$.
Like the main-paper exact anchor, it uses no continuation, and remaining spans follow in decreasing probability.

The enumerate-and-cover order starts empty. At each step, it adds the span that newly matches candidates with the largest total model probability at tIoU $\tau$.
With $U_k$ denoting candidates already matched at step $k$, we select
\begin{equation}
y_k\in\arg\max_y
\sum_{y'\notin U_k:\ \operatorname{tIoU}(y,y')\ge\tau}p_f(y'\mid X).
\label{eq:supp:cover-order}
\end{equation}
After reaching model-estimated success 0.999 or selecting 300 spans, it appends the rest in probability order.
Calibration and prediction remain unchanged.

At threshold $q$, per-second thresholding builds a region directly, keeping each whole second whose model-estimated marginal probability of lying inside a candidate moment is at least $1-q$.
The three anchor families each use eight $q_0$ values, giving 24 configurations.
Enumerate-and-cover and per-second thresholding add one each because neither uses $q_0$, giving 26 in total.
The gain-per-second anchor, enumerate-and-cover order and per-second thresholding do not require $\tau\ge1/2$.
For $\tau<1/2$, the gain-per-second anchor can replace the exact anchor, and \cref{thm:validity} still gives marginal coverage; all reported experiments use $\tau\ge1/2$.

\paragraph{Choosing $q_0$ and the watched-region type.}
For each candidate $q_0$ in the main-paper configuration, we calibrate a temporary split-conformal threshold on the fit queries.
We choose the $q_0$ with the lowest mean watch duration on those queries, discard its threshold, and calibrate on independent videos.

For supplementary selection, we randomly split the fit videos in half 100 times.
One query sampled uniformly per video in the first half calibrates all 26 configurations.
The second half measures watch duration, and we choose the configuration with the lowest mean across splits.
Neither procedure uses the final calibration set.

\paragraph{From calibration scores to prediction.}
For each calibration query, we add spans in order until the watched region first contains a matching clip.
The score is the model-estimated success probability immediately before that step, or 1 if no prefix of the retained pool succeeds.
For $q<1$, prediction returns the first prefix with model-estimated success above $q$, which misses exactly when the score exceeds $q$.
At $q=1$, it returns the uncapped full pool and hence the entire video.

We sample one query uniformly from each of $n$ calibration videos and set $k_n=\lceil(n+1)(1-\alpha)\rceil$.
The threshold $\hat q$ is the $k_n$-th smallest score when $k_n\le n$, and 1 otherwise.
A selected score of 1 also triggers the full-pool fallback.
\Cref{tab:supp:units} tests the importance of using videos as units.

\subsection{Comparison methods and annotation handling}
\label{sec:supp:impl:baselines}

\paragraph{Prior conformal grounding.}
The prior method, COVER~\cite{mohamed2026cover}, widens one base answer span to contain the whole annotated moment, with a marginal guarantee over queries.
When several moments are annotated, it targets their temporal hull, from the earliest start to the latest end.
It has no tIoU parameter.
We use the greedy answer's span as this base span, taking the longest one when the answer has several, denoted $[\hat s,\hat e]$ with length $\ell$.
For annotation hull $[s^\star,e^\star]$, its normalized calibration score is $\max\{(\hat s-s^\star)/\ell,(e^\star-\hat e)/\ell\}$.
With $N_{\mathrm{cal}}$ calibration queries, we set $\hat\mu$ to the $\lceil(N_{\mathrm{cal}}+1)(1-\alpha)\rceil$-th smallest score.
The returned region is $[\hat s-\hat\mu\ell,\hat e+\hat\mu\ell]\cap[0,T]$.
If the model refuses to answer, it returns $[0,T]$.
Calibration treats individual queries as exchangeable units.

\paragraph{Single answers and calibrated scales.}
MBR over all spans selects the whole-second span with highest expected tIoU under $p_f(\cdot\mid X)$.
The MBR answer at $\tau$ instead maximizes the model-estimated probability of matching a candidate moment at tIoU $\tau$.
The calibrated greedy and MBR answers in \cref{tab:methods} expand or shrink about their centers, then clip to $[0,T]$.
They use scales $\{0,0.1,\dots,2,2.5,3,4,5,7,10,15,20,30,50,100,\infty\}$, where $\infty$ returns the entire video.
As in \texttt{CAPTURE}, video-level split-conformal calibration selects the scale.
A query's score is the smallest scale whose region contains a matching clip.
We sample one query uniformly per calibration video and choose the $k_n$-th smallest score as the calibrated scale.
If no valid greedy answer exists, the calibrated greedy answer returns the entire video.
The main paper labels the calibrated greedy and MBR answers \texttt{CAPTURE}, greedy anchor and \texttt{CAPTURE}, MBR anchor at $\tau$.

\paragraph{Positional prior.}
This baseline uses the annotated moments' typical locations in the fit videos.
We divide relative position $t/T$ into 100 bins.
For each fit query and bin, we add the proportions of the bin covered by each moment and cap the sum at 1.
Averaging these capped values over fit queries gives the bin's prior.
At threshold $\lambda$, the region includes each whole second whose center lies in a bin with prior at least $\lambda$.
The same video-level split-conformal procedure selects $\lambda$, ordering thresholds so that decreasing $\lambda$ only enlarges the region.

\paragraph{Annotations outside the video.}
Of ActivityNet Captions' 5,675 moments, 937 end up to 0.05 seconds beyond the video boundary and cannot be contained by any interval inside $[0,T]$.
We clip these 937 annotations when measuring whole-moment containment and the overlap measures in \cref{tab:supp:quality}.
