# Supplementary material for: CAPTURE: Minimizing Watch Time for Reliable Temporal Video Grounding
Source: arXiv:2611.38466 source file (2026-11-28)
Supplement: Supplementary file 5 [file proofs.tex]

\section{Proofs}
\label{sec:supp:proofs}

\texttt{CAPTURE} first constructs an anchor using the model probabilities, then calibrates how much of it to return or how far to expand it.
We prove marginal coverage, show how the dynamic program finds an exact anchor, and establish the watch-duration bound in Theorem~1.
We then prove that model errors make the higher oracle success level necessary and explain why containing a matching clip does not ensure that the region itself has high tIoU.

\begin{restatedtheorem}{thm:main}[Coverage and watch-duration guarantee]
Suppose Assumptions~\ref*{ass:xchange} and
\ref*{ass:real} hold. For any $q_0\in[0,1]$
fixed independently of calibration data,
the prediction set $\widehat C(X_{\mathrm{test}})$
returned by \texttt{CAPTURE} satisfies
\begin{equation}
\Pr\bigl(
a_\tau(\widehat C(X_{\mathrm{test}}),
Y_{\mathrm{test}})=1
\bigr)\ge1-\alpha.
\tag{\ref*{eq:coverage_guarantee}}
\end{equation}

Furthermore, suppose Assumptions~\ref*{ass:model}
and \ref*{ass:oracle} also hold. Let
$\delta\in(0,1)$ and
$k_n=\lceil(n+1)(1-\alpha)\rceil\le n$.
If $q_0$ satisfies
\begin{equation}
q_0\ge
\frac{k_n}{n}+\epsilon_A+
\sqrt{\frac{\log(1/\delta)}{2n}},
\qquad q_0+\epsilon_L\le1,
\tag{\ref*{eq:q0_condition}}
\end{equation}
then
\begin{equation}
\Pr\bigl(
W(\widehat C(X_{\mathrm{test}}))
\le \operatorname{OPT}_P(
X_{\mathrm{test}},q_0+\epsilon_L)
\bigr)
\ge1-\delta-\beta,
\tag{\ref*{eq:watch_duration_guarantee}}
\end{equation}
where the probabilities are taken over randomness in calibration and test
data.
\end{restatedtheorem}

\begin{proof}[Proof of Theorem~1]
We prove both claims below for calibration with independent videos.
Assumption~\ref*{ass:xchange} is the special case in which each video has one query.
With $h=a_\tau$, \cref{thm:validity} gives marginal coverage and \cref{thm:watch} gives the watch-duration bound.
Assumption~\ref*{ass:real} ensures that the full pool succeeds almost surely, as required for coverage.
\Cref{thm:validity} also requires $Q(\cdot\mid x)$ to sum to 1 over $\mathcal P$ and candidate spans to have positive length, which holds for the renormalized whole-second spans used throughout (\cref{sec:supp:impl:scoring}).
The proofs also allow the region success rule used in the experiments.
\end{proof}

\paragraph{Calibrating with videos as units.}
Different queries about the same video can lead to related model errors.
They share visual content, and their annotations may come from the same annotators and procedure.
We therefore draw one query uniformly from each of $n$ independent calibration videos and sample the test query in the same way from a new video.
This permits dependence within a video without assuming that all queries are exchangeable (\cref{tab:supp:units}).
The calibration and test videos, together with their queries and annotations, are i.i.d.\ and independent of the fit videos $\mathcal D_{\mathrm{fit}}$, which form the validation set of the main paper.
The fit videos determine the model-estimated success threshold $q_0$ and, for the variants in \cref{sec:supp:impl:regions}, the watched-region type before calibration.
Let $P$ denote the resulting distribution of input--annotation pairs $(X,Y)$.

\paragraph{What counts as a successful prediction.}
The main paper distinguishes selecting a matching span from returning footage that contains a matching clip.
For input $X$, prediction set $C$ and annotation $Y$, let $h(C,Y)=1$ for success and 0 otherwise.
Under the \emph{span-set rule}, $h=a_\tau$ requires at least one selected span to match a ground-truth moment at tIoU $\tau$ (\cref{eq:admit}).
Under the \emph{region rule}, any clip $s\subseteq R(C)$ can establish success if $\operatorname{tIoU}(s,y)\ge\tau$ for some $y\in Y$.
That clip need not itself be selected.
Adding spans cannot turn a success into a failure under either rule.
Also, a matching selected span always lies in the watched region, so $h(C,Y)\ge a_\tau(C,Y)$.
These two properties allow the coverage and watch-duration proofs to apply to both rules under their stated assumptions.

A prefix contains the first several spans in the fixed ordering.
Line~6 of \cref{alg:capture_calibration} tests whether a selected span matches.
The experiments instead test whether the watched region contains a matching clip when finding the first successful prefix $j_i^\star$ (\cref{sec:capture_algorithm,sec:exp}).
Only this test of calibration success changes with $h$.
The probabilities $U_P$ and $U_Q$ still use the span-set rule (\cref{eq:true_utility,eq:model_utility}), as do the oracle $\mathrm{OPT}_P$ (\cref{eq:opt}) and model errors $e_\pm$ (\cref{eq:overestimation_error,eq:underestimation_error}).
For requested success rate $1-\alpha$, we require
\begin{equation}
\Pr\big(h(\widehat C(X),Y)=1\big)\ge1-\alpha.
\label{eq:goal}
\end{equation}
The probability includes calibration and test videos, sampled queries and independent tie-breaking randomness.
With $h=a_\tau$, \cref{eq:goal} is \cref{eq:coverage_guarantee}.

\subsection{Validity of \texttt{CAPTURE}}
\label{sec:supp:proofs:validity}

Calibration chooses how many ordered spans to return.
Each calibration score is the model-estimated success probability just before the first successful prefix.
Prediction returns the first prefix whose probability exceeds the calibrated threshold, or the full pool if the threshold is 1.
For the proof, we also define a test score using the unknown test annotation.
If the threshold reaches that score, prediction cannot stop before the first successful prefix.
The split-conformal rank argument makes this happen with probability at least $1-\alpha$ when the full pool succeeds~\cite{papadopoulos2002inductive,vovk2005algorithmic,lei2018distribution}.
The theorem also accounts for cases where the full pool fails.

\begin{theorem}[Marginal coverage with videos as units]
\label{thm:validity}
Fix $\tau\in(0,1]$ and $\alpha\in(0,1)$.
Condition on the fit videos, fixing the grounding model, candidate-pool construction, ordering rule and $q_0\in[0,1]$.
Assume that calibration and test videos, including all their queries and annotations, are i.i.d.\ and independent of the fit videos.
For every input $x$, let $Q(\cdot\mid x)$ sum to 1 over $\mathcal P$, and let every candidate span have positive length.
Draw one query uniformly at random from each calibration video and from the test video.
Run \cref{alg:capture_calibration} on the $n$ calibration queries and \cref{alg:capture_prediction} on the test query, using $h$ in place of $a_\tau$ to test prefix success in \cref{alg:capture_calibration}.

First suppose that the full candidate pool succeeds almost surely, meaning that
$\Pr(h(\mathcal P,Y)=1)=1$.
When $h=a_\tau$, this condition is Assumption~\ref*{ass:real}.
Then the test prediction satisfies \cref{eq:goal}.

If instead the full pool fails with probability $p_0:=\Pr(h(\mathcal P,Y)=0)$, assign score 1 whenever no prefix succeeds.
Marginal coverage is then at least $1-\alpha-p_0$.
\end{theorem}

\begin{proof}
Condition on the fit videos, fixing the model, candidate-pool and anchor constructions, ordering rule and $q_0$.

\emph{Step 1. Apply the same sampling and scoring rules to every video.}
Write $\mathcal V_v$ for video $v$ with its queries and annotations, where $v\le n$ denotes calibration and $v=n+1$ testing.
Conditional on $\mathcal V_v$, draw query index $\iota_v$ uniformly and denote its input and annotation by $(X_v,Y_v)$.
Sampling randomness is independent across videos and independent of video records and tie-breaking noise.
For randomized tie-breaking, draw $\xi_v$ from a fixed distribution, independently across videos and independently of the data.
Use the same function of $(X_v,\xi_v)$ for every video.
For deterministic tie-breaking, omit $\xi_v$.
The video records are i.i.d., and every video uses the same sampling rule.
Thus the triples $(\mathcal V_v,\iota_v,\xi_v)$ are i.i.d., as are the sampled examples
$(X_1,Y_1,\xi_1),\dots,(X_{n+1},Y_{n+1},\xi_{n+1})$.
In particular, $(X_v,Y_v)\sim P$ satisfies Assumption~\ref*{ass:xchange}.

Let $C_j(X_v)$ contain the first $j$ ordered spans, with model-estimated success $u_j(X_v)$.
The anchor, ordering and these values are fixed functions of $(X_v,\xi_v)$.
Let $j_v^\star$ denote the first successful prefix, so $h(C_{j_v^\star}(X_v),Y_v)=1$.
Its score is $Z_v=u_{j_v^\star-1}(X_v).$
The same scoring rule gives i.i.d.\ scores $Z_1,\dots,Z_{n+1}$.
They are therefore exchangeable, meaning that relabeling them leaves their joint distribution unchanged.
Because the full pool succeeds, a first successful prefix $j_v^\star\le N$ exists.
Since each $u_j$ is a probability, $Z_v\in[0,1]$.

\emph{Step 2. Reaching the test score ensures success.}
At $\hat q=1$, \cref{alg:capture_prediction} returns the full pool $\mathcal P$, which succeeds almost surely.
Now suppose $\hat q<1$.
Although $h$ determines success against $Y_{n+1}$, the model-estimated probability $U_Q$ still uses $a_\tau$.
Every positive-length candidate matches itself because its tIoU with itself is 1 for every $\tau\in(0,1]$.
Since $Q(\cdot\mid X_{n+1})$ sums to 1, $u_N(X_{n+1})=1>\hat q$.
When we cap the pool, we renormalize the retained probabilities to sum to 1 (\cref{sec:supp:impl:scoring}).
The first prefix above the threshold therefore exists,
$\hat j=\min\{j:u_j(X_{n+1})>\hat q\}$.

Suppose $Z_{n+1}\le\hat q$, where $Z_{n+1}=u_{j_{n+1}^\star-1}(X_{n+1})$.
Adding spans preserves matched candidates, so model-estimated success is nondecreasing and
\[
u_j(X_{n+1})
\le
u_{j_{n+1}^\star-1}(X_{n+1})
=
Z_{n+1}
\le\hat q,
\qquad
j\le j_{n+1}^\star-1.
\]
No prefix before the first success exceeds the threshold.
Thus $\hat j\ge j_{n+1}^\star$, and $C_{\hat j}(X_{n+1})$ contains the successful prefix $C_{j_{n+1}^\star}(X_{n+1})$.
Monotonicity of $h$ makes the returned prediction successful.

\emph{Step 3. The threshold reaches the test score often enough.}
Let $k_n=\lceil(n+1)(1-\alpha)\rceil$.
If $k_n>n$, then $\hat q=1$ and Step 2 gives success with probability 1.
Otherwise $k_n\le n$.
Write $k=k_n$ and set $\hat q=Z_{(k)}$, the $k$-th smallest calibration score.
To apply exchangeability, include the test score $Z_{n+1}$ and let $Z_{(k)}^{+}$ be the $k$-th smallest of all $n+1$ scores.
Adding a score cannot increase that value, so $Z_{(k)}^{+}\le Z_{(k)}=\hat q.$
Consequently, $Z_{n+1}\le Z_{(k)}^{+}$ implies $Z_{n+1}\le\hat q$.

At least $k$ scores are at most $Z_{(k)}^{+}$, and ties can only increase this count.
By exchangeability, each score has the same probability $p$ of satisfying $Z_i\le Z_{(k)}^{+}$.
The expected count is therefore $(n+1)p\ge k$.
In particular, the test score satisfies $\Pr\bigl(Z_{n+1}\le Z_{(k)}^{+}\bigr)\ge \frac{k}{n+1}.$
Since $Z_{(k)}^{+}\le\hat q$ and $k=k_n\ge(n+1)(1-\alpha)$,
\[
\Pr(Z_{n+1}\le\hat q)
\ge
\frac{k}{n+1}
\ge
1-\alpha.
\]
Step 2 converts this bound into \cref{eq:goal}.

\emph{Step 4. Account for full-pool failures.}
Allow full-pool failure with probability $p_0=\Pr(h(\mathcal P,Y)=0)$ and assign score 1 whenever no prefix succeeds.
The common scoring rule preserves exchangeability.
If $k_n>n$, then $\hat q=1$ returns the full pool and succeeds with probability $1-p_0$.
Otherwise Step 3 still gives $\Pr(Z_{n+1}\le\hat q)\ge1-\alpha.$
Here $\hat q=Z_{(k_n)}$ can equal 1.
If $Z_{n+1}\le\hat q$ and $h(\mathcal P,Y)=1$, prediction succeeds by Step 2 for $\hat q<1$, or by returning the full pool for $\hat q=1$.
Thus only full-pool failure can prevent success when the threshold reaches the test score.
Subtracting its probability gives
\[
\Pr(Z_{n+1}\le\hat q)-\Pr(h(\mathcal P,Y)=0)
\ge 1-\alpha-p_0.
\]
\end{proof}

\paragraph{Tie-breaking randomness.}
Tie-breaking may be deterministic or use independent noise from a fixed distribution, independent of the data.
GPU summation order need not satisfy these assumptions (\cref{sec:supp:proofs:dp}).

\paragraph{Choices made with the fit videos.}
Fit videos determine $q_0$, region type and comparison-method settings independently of calibration.
The rank argument applies when each prediction contains the preceding one and the largest succeeds almost surely.
For \texttt{CAPTURE}, this requires $h(\mathcal P,Y)=1$ almost surely.
For calibrated scales and the positional prior, the largest prediction is the whole video.

\paragraph{When no prediction in a family succeeds.}
For methods calibrated over a grid, we order grid values from smaller to larger prediction sets.
The score is the first value whose prediction succeeds, or $+\infty$ if none does.
\texttt{CAPTURE} uses score 1 for failure because its scores are model-estimated probabilities.
A calibrated threshold of 1 returns the full pool.

\subsection{The exact anchor}
\label{sec:supp:proofs:dp}

We find the shortest region reaching model-estimated success $q_0$, then construct its anchor from candidate spans inside it (\cref{sec:supp:proofs:watch}).
For the exact computation, the video duration $T$ and watched-segment endpoints are integer seconds.
For non-integer $T$, the same program on $[0,\lfloor T\rfloor]$ covers every whole-second candidate span.
We merge touching or overlapping segments, leaving a region $R$ whose segments are separated by at least one second.
Its watch duration $|R|$ is the sum of their lengths.
A matching clip $s$ inside the region may have arbitrary endpoints and need not be selected from the candidate pool.

The model treats each candidate $y$ as a possible moment with probability $p_f(y\mid X)=Q(y\mid X)$.
We count this probability once whenever $R$ contains a clip matching $y$,
\begin{equation}
U_f(R\mid X)=\sum_y p_f(y\mid X)\,
\mathbf 1\{\exists s\subseteq R:\ \operatorname{tIoU}(s,y)\ge\tau\}.
\label{eq:ucov}
\end{equation}
This region-rule estimate allows any matching clip inside $R$, whereas $U_Q$ in \cref{eq:model_utility} requires a selected span to match.
We minimize watch duration subject to reaching $q_0$,
\begin{equation}
R^\star(X)\in\operatorname*{arg\,min}_{R:\,U_f(R\mid X)\ge q_0}|R|.
\label{eq:anchor}
\end{equation}
Ties may be resolved arbitrarily.
The non-strict constraint permits $q_0=1$.
For variants requiring $U_f(R\mid X)>q_0$, the same proof applies with a strict inequality and $q_0<1$.

\paragraph{Idea of the dynamic program.}
For any watch-duration budget, we want the region with the highest model-estimated success probability.
The dynamic program builds the region from left to right, choosing which parts to watch or skip.
The key property is that, for $\tau\ge1/2$, two separated segments cannot both contain clips matching the same candidate moment.
We can therefore add their contributions without counting a candidate's probability twice.

Let $c(G)$ denote the total model probability of candidates matched by a clip inside segment $G$, with $c(a,b)$ used for $G=[a,b]$.
Define $F_t(w)$ as the highest success probability achievable inside $[0,t]$ using at most $w$ seconds.
To compute it, we compare skipping $[t-1,t]$ with watching a final segment $[a,t]$ for every possible start $a<t$.
After reaching the video end, the smallest $w$ with $F_T(w)\ge q_0$ gives the minimum watch duration.
Tracing the stored choices backward recovers the region (\cref{fig:supp:dp}).
For $\tau<1/2$, two segments may both match the same candidate, so their contributions need not add and the recurrence is no longer exact.

\input{fig/dp}

\begin{algorithm*}[t]
\caption{Exact minimum-watch-duration region}
\label{alg:watch}
\small
\begin{algorithmic}[1]
\Require probabilities $p_f(y\mid X)$ for all positive-length spans $y$ with integer endpoints in $[0,T]$, tIoU threshold $\tau\ge1/2$, model-estimated success threshold $q_0$
\Ensure region $R^\star(X)$, a set of disjoint segments
\Statex \textit{Step 1. Value of each single segment}
\For{each segment $[a,b]$ with $0\le a<b\le T$}
\State $c(a,b)\gets\sum_{y}p_f(y\mid X)\,\mathbf 1\{|y\cap[a,b]|\ge\tau|y|\}$
\EndFor
\Statex \textit{Step 2. Sweep from left to right}
\State $F_{-1}(w)\gets0$, $\ F_0(w)\gets0$ for $w=0,\dots,T$
\For{$t=1,\dots,T$ and $w=0,\dots,T$}
\State $F_t(w)\gets F_{t-1}(w)$, $\ B_t(w)\gets\varnothing$ \Comment{skip second $t$}
\For{$a=\max\{0,t-w\},\dots,t-1$} \Comment{segment $[a,t]$}
\State $v\gets F_{a-1}\big(w-(t-a)\big)+c(a,t)$ \Comment{gap of one second}
\State \textbf{if} $v>F_t(w)$ \textbf{then} $F_t(w)\gets v$, $\ B_t(w)\gets a$
\EndFor
\EndFor
\Statex \textit{Step 3. Least watch duration and traceback}
\State $w\gets\min\{w':F_T(w')\ge q_0\}$, $\ t\gets T$, $\ R\gets\varnothing$
\While{$t>0$}
\State \textbf{if} $B_t(w)=\varnothing$ \textbf{then} $t\gets t-1$ \Comment{second $t$ not watched}
\State \textbf{else} $a\gets B_t(w)$, add $[a,t]$ to $R$, $w\gets w-(t-a)$, $t\gets a-1$
\EndWhile
\State \Return $R^\star(X)=R$
\end{algorithmic}
\end{algorithm*}

\begin{proposition}[Exact minimum-watch-duration region]
\label{prop:dp}
For $\tau\ge1/2$, \cref{alg:watch} returns a region that solves \cref{eq:anchor} and requires $O(T^3)$ operations when Step 1 uses cumulative sums.
\end{proposition}

\begin{proof}
\emph{Step 1. Determine when a segment contains a matching clip.}
Fix a segment $G$ and candidate $y\in\mathcal P$.
If $|y\cap G|\ge\tau|y|$, choose the clip $s=y\cap G$.
Since $s\subseteq y$, $\operatorname{tIoU}(s,y) =\frac{|y\cap G|}{|y|} \ge\tau.$
Conversely, a clip $s\subseteq G$ cannot overlap $y$ more than $G$ does.
Its union $s\cup y$ also cannot be shorter than $y$.
Thus
\[
\operatorname{tIoU}(s,y)
\le\frac{|s\cap y|}{|y|}
\le\frac{|G\cap y|}{|y|}.
\]
If $|G\cap y|<\tau|y|$, no clip inside $G$ can match $y$.
Thus $G$ contains a matching clip exactly when $|y\cap G|\ge\tau|y|$.
Summing $p_f(y\mid X)$ over these candidates gives $c(G)$, or $c(a,b)$ for $G=[a,b]$, in Step 1 of \cref{alg:watch}.

\emph{Step 2. Add segment contributions without counting a candidate twice.}
Let $G_1,\ldots,G_\nu$ be the separate watched segments in $R$.
A clip inside $R$ cannot cross an unwatched gap.
By Step 1, a matching clip exists exactly when some segment satisfies $|y\cap G_k|\ge\tau|y|$.
If $y$ intersects two segments, it also contains their gap of at least one second, so $\sum_k |y\cap G_k|\le |y|-1.$
For both segments to contain matching clips, each would need overlap $\tau|y|\ge|y|/2$.
Their total overlap would then be at least $2\tau|y|\ge|y|$, a contradiction.
Hence $\sum_k\mathbf 1\{|y\cap G_k|\ge\tau|y|\}$ is zero or one and equals the region's success indicator.
Multiplying by $p_f(y\mid X)$ and summing gives $U_f(R\mid X)=\sum_k c(G_k),$ with no probability counted twice.

\emph{Step 3. Show that the recurrence finds the optimum.}
Let $\Phi_t(w)$ be the largest $\sum_k c(G_k)$ attainable inside $[0,t]$ with total duration at most $w$ and gaps of at least one second.
We prove $F_t(w)=\Phi_t(w)$ by induction on $t$.
At $t=-1$ and $t=0$, only the empty collection is possible, so $\Phi_{-1}(w)=\Phi_0(w)=0$, matching initialization.
For $t\ge1$, there are two possibilities.
If the last second is skipped, the best value is $\Phi_{t-1}(w)$ inside $[0,t-1]$.
Otherwise the final component is some $[a,t]$, using $t-a$ seconds and contributing $c(a,t)$.
Earlier components must end by $a-1$, leaving the required gap, and use at most $w-(t-a)$ seconds.
Their best contribution is $\Phi_{a-1}(w-(t-a))$, which equals $F_{a-1}(w-(t-a))$ by induction.
Step 2 of \cref{alg:watch} compares these choices for every feasible $a$.
These choices cover every feasible collection and use the correct earlier optima, so $F_t(w)=\Phi_t(w)$.
At $t=T$, these collections give all feasible watched regions, and Step 2 gives
\[
F_T(w)=\max\{U_f(R\mid X):|R|\le w\}.
\]
Watching the entire video succeeds under the model because every candidate matches itself and probabilities sum to 1.
Hence $F_T(T)=1\ge q_0$, and the smallest $w^\star$ with $F_T(w^\star)\ge q_0$ is the minimum in \cref{eq:anchor}.
Backward tracing returns a region of duration $w^\star$ meeting the threshold.
For a strict constraint, replace $\ge$ by $>$ and require $q_0<1$.

\emph{Step 4. Count the operations.}
Each of the $O(T^2)$ entries $(t,w)$ examines $O(T)$ starts $a$, giving $O(T^3)$ operations.
Computing segment values has the same cost.
For a candidate $y=[y_s,y_e]$, a segment starting at $a$ can contain a matching clip only if $a\le y_e-\tau|y|.$
If $a>y_e-\tau|y|$, extending the segment beyond $y_e$ still leaves less than $\tau|y|$ overlap.
Otherwise, every integer end $b\ge\max\{a,y_s\}+\tau|y|$ provides enough overlap.
The first such end is $b=\left\lceil\max\{a,y_s\}+\tau|y|\right\rceil$.
We record the candidate's probability there in a difference array and use cumulative sums over $b$ to include it at every later end.
The $O(T^2)$ candidates and $O(T)$ starts per candidate require $O(T^3)$ updates.
The cumulative sums do not increase this order, so Step 1 and the recurrence both cost $O(T^3)$.
\end{proof}

GPU reductions may sum probabilities in different orders.
Floating-point addition is not exactly associative, so mathematically tied values can differ slightly and change tie-breaking for the continuation and gain-per-second anchors.
Across repeated runs, a table cell's mean normalized watch duration changed by at most about 0.001.
Runtime is reported in \cref{tab:supp:runtime}.

\subsection{The watch-duration bound}
\label{sec:supp:proofs:watch}

We compare the final prediction with the oracle $\mathrm{OPT}_P(x,r)$, which minimizes watch duration among prediction sets with true conditional success probability at least $r$.
The proof has two parts.

First, calibration must stop within the anchor.
If overestimation is at most $\epsilon_A$ on average, choosing $q_0$ as in \cref{eq:q0_condition} makes enough calibration anchors succeed with high probability.
Inclusion-minimality puts each successful anchor's score below $q_0$.
The calibrated threshold then stays below $q_0$, keeping prediction within the anchor.

Second, the anchor must be no longer than the oracle.
If $e_-(x)\le\epsilon_L$, an oracle set with true success at least $q_0+\epsilon_L$ still reaches model-estimated success $q_0$.
An exact anchor cannot be longer than this feasible set.
Assumption~\ref*{ass:model} gives this condition with probability at least $1-\beta$ over test inputs.

The argument applies at any tIoU threshold when $A_0(x)$ solves \cref{eq:oracle} exactly and removing redundant spans makes $A(x)$ inclusion-minimal.
The dynamic program in \cref{sec:supp:proofs:dp} provides this anchor for $\tau\ge1/2$ over all positive-length integer-endpoint spans.

\begin{theorem}[Watch duration with videos as calibration units]
\label{thm:watch}
Assume the conditions of \cref{thm:validity}, and let the anchor satisfy Assumption~\ref*{ass:oracle}.
Let Assumption~\ref*{ass:model} hold under $P$, with constants $\epsilon_A$, $\epsilon_L$ and $\beta$.
Let $\delta\in(0,1)$ and $k_n=\lceil(n+1)(1-\alpha)\rceil\le n$, and let $q_0$ satisfy \cref{eq:q0_condition}.
With probability at least $1-\delta$, every input $x$ satisfying $e_-(x)\le\epsilon_L$ obeys
\[
W(\widehat C(x))\le\mathrm{OPT}_P(x,q_0+\epsilon_L).
\]
This probability is over the calibration videos, their query draws and any calibration-time tie-breaking randomness, and the bound holds simultaneously for all such inputs.
In particular, the prediction for a uniformly sampled query from the test video satisfies \cref{eq:watch_duration_guarantee}.
\end{theorem}

\begin{proof}
Condition on the fit videos, fixing the model, $q_0$, anchor rule and all other fitted choices.

\emph{Step 1. Bound how often calibration anchors succeed.}
For calibration video $v$, define $H_v=h(A(X_v),Y_v).$
This is 1 if the anchor for its sampled query succeeds and 0 otherwise.
The sampled pairs are independent draws from $P$ and use the same anchor rule and success test.
Thus $H_1,\ldots,H_n$ are i.i.d.\ Bernoulli variables, and their common mean $\mathbb E H_v$ is the anchor's success probability.
For every input and annotation, $h(A(X),Y)\ge a_\tau(A(X),Y)$, with equality for $h=a_\tau$.
For the region rule, a matching selected span also supplies a matching clip.
For fixed $X$ and independent tie-breaking noise, the anchor is fixed.
Its probability of span-set success over possible annotations is $U_P(A(X)\mid X)$.
Averaging over inputs and tie-breaking therefore gives $\mathbb E H_v\ge \mathbb E\,U_P(A(X)\mid X).$

Overestimation bounds the difference between the model and true success probabilities,
\[
U_P(A(X)\mid X)
\ge U_Q(A(X)\mid X)-e_+(X).
\]
Removing redundant spans preserves $U_Q(A(X)\mid X)\ge q_0$, so $U_P(A(X)\mid X)\ge q_0-e_+(X).$
Taking expectations with $\mathbb E e_+(X)\le\epsilon_A$ yields $\mathbb E H_v\ge q_0-\epsilon_A.$
This averages over queries, annotations and tie-breaking randomness.

\emph{Step 2. Ensure enough anchors succeed in the calibration sample.}
The observed success rate may fall below its mean.
Set $\gamma=\sqrt{\frac{\log(1/\delta)}{2n}}.$
Hoeffding's inequality bounds the probability of a downward deviation of at least $\gamma$ by $\exp(-2n\gamma^2)=\delta.$
Since $\mathbb E H_v\ge q_0-\epsilon_A$,
\[
\Pr\left(
\frac1n\sum_{v=1}^nH_v
\le q_0-\epsilon_A-\gamma
\right)\le\delta.
\]
Thus, with probability at least $1-\delta$, $\sum_{v=1}^nH_v >n(q_0-\epsilon_A-\gamma).$
The lower bound on $q_0$ in \cref{eq:q0_condition} is equivalent to $n(q_0-\epsilon_A-\gamma)\ge k_n.$
At least $k_n$ anchors therefore succeed on this event.
The required margin covers both average overestimation $\epsilon_A$ and sampling deviation $\gamma$.

\emph{Step 3. A successful anchor gives a score below $q_0$.}
We now relate a successful anchor to its calibration score.
For fixed $x$, examine $A_0(x)$ from lowest to highest model probability, removing $s$ from the current set $S$ if $U_Q(S\setminus\{s\}\mid x)\ge q_0$.
Keeping $s$ means $U_Q(S\setminus\{s\}\mid x)<q_0.$
Later deletions leave $A(x)\setminus\{s\}\subseteq S\setminus\{s\}$ and cannot increase $U_Q$, so
\[
U_Q(A(x)\setminus\{s\}\mid x)<q_0
\qquad\text{for every }s\in A(x).
\]
For any proper subset $C\subsetneq A(x)$, choose $s\in A(x)\setminus C$.
Then $C\subseteq A(x)\setminus\{s\}$, giving
\[
U_Q(C\mid x)
\le U_Q(A(x)\setminus\{s\}\mid x)
<q_0.
\]
Every proper subset therefore has model-estimated success probability below $q_0$, establishing inclusion-minimality.

Since \cref{eq:q0_condition} implies $q_0>0$ and $U_Q(\varnothing\mid x)=0$, every anchor has $d(x)=|A(x)|\ge1$ spans.
These come first in the ordering.
If $H_v=1$, a prefix succeeds by the time the entire anchor is selected, so $j_v^\star\le d(X_v)$.
The preceding prefix is a proper subset of the anchor, giving
\[
Z_v
=U_Q(C_{j_v^\star-1}(X_v)\mid X_v)
<q_0.
\]

\emph{Step 4. The prediction stops within the anchor.}
On the event established in Step 2, at least $k_n$ anchors succeed.
Step 3 shows that each has a score below $q_0$.
The $k_n$-th smallest calibration score $\hat q=Z_{(k_n)}$ therefore satisfies $\hat q<q_0\le1.$
For every test input $x$, its first $d(x)$ spans form the anchor and
\[
u_{d(x)}(x)=U_Q(A(x)\mid x)\ge q_0>\hat q.
\]
The first prefix above $\hat q$ must therefore satisfy $\hat j(x)\le d(x).$
Consequently,
\[
\widehat C(x)\subseteq A(x),
\qquad
W(\widehat C(x))\le W(A(x)),
\]
which is \cref{eq:anchor_containment}.

\emph{Step 5. Compare the anchor with the true oracle.}
Fix $x$ with $e_-(x)\le\epsilon_L$.
Suppose some prediction set reaches true success probability $q_0+\epsilon_L$.
Since the candidate pool is finite, an optimal set $C^\star$ attains $\mathrm{OPT}_P(x,q_0+\epsilon_L)$ and satisfies $U_P(C^\star\mid x)\ge q_0+\epsilon_L.$
Since the model underestimates success by at most $\epsilon_L$,
\[
U_Q(C^\star\mid x)
\ge U_P(C^\star\mid x)-e_-(x)
\ge q_0.
\]
Thus $C^\star$ is feasible for \cref{eq:oracle}.
The exact optimum $A_0(x)$ obeys $W(A_0(x))\le W(C^\star).$
Removing redundant spans gives $W(A(x))\le W(A_0(x)).$
Combining these comparisons,
\[
W(A(x))
\le W(A_0(x))
\le W(C^\star)
=\mathrm{OPT}_P(x,q_0+\epsilon_L).
\]

If no span set meets the oracle request, $\mathrm{OPT}_P(x,q_0+\epsilon_L)=+\infty$, and the inequality gives no finite duration bound.
For $h=a_\tau$, almost-sure full-pool success in \cref{thm:validity} gives $U_P(\mathcal P\mid x)=1$ for $P_X$-almost every $x$.
Together with $q_0+\epsilon_L\le1$ from \cref{eq:q0_condition}, this makes the oracle feasible almost everywhere.
Under the region rule, the full pool may contain a matching clip even when none of its spans matches.
The span-set oracle can then be infeasible, in which case we use the same $+\infty$ convention.

\emph{Step 6. Combine the two probability bounds.}
With probability at least $1-\delta$ over calibration, Steps 4 and 5 give the comparison simultaneously for all $x$ with $e_-(x)\le\epsilon_L$.
Assumption~\ref*{ass:model} gives this condition with test probability at least $1-\beta$.
Failure requires either the calibration event to fail or $e_-(X)>\epsilon_L$.
A union bound limits its probability to $\delta+\beta$, proving \cref{eq:watch_duration_guarantee}.
\end{proof}


\paragraph{Which model errors the proof needs.}
Step 1 only controls overestimation for the anchor.
The weaker condition
\[
\mathbb E\big(U_Q(A(X)\mid X)-U_P(A(X)\mid X)\big)_+
\le\epsilon_A
\]
therefore suffices in place of $\mathbb E e_+(X)\le\epsilon_A$, which controls all span sets.
Steps 2--4 still give $\hat q<q_0$ with probability at least $1-\delta$ and hence \cref{eq:anchor_containment}.
\Cref{sec:supp:bound:practice} examines measured model errors and the extra margin needed with finitely many calibration videos.

Algorithm~\ref{alg:s:capture} converts the optimal region into an optimal span set.
We next show that this satisfies Assumption~\ref*{ass:oracle}.

\begin{algorithm*}[t]
\caption{\texttt{CAPTURE} with the exact anchor and videos as calibration units}
\label{alg:s:capture}
\small
\begin{algorithmic}[1]
\Require probabilities $p_f(\cdot\mid X)$ over all positive-length integer-endpoint spans in $[0,T]$, tIoU threshold $\tau\ge1/2$, success indicator $h$, model-estimated success threshold $q_0$ selected on the fit videos, requested success rate $1-\alpha$, and calibration videos $v=1,\dots,n$
\Ensure prediction set $\widehat C(X)\subseteq\mathcal P$ for each test input
\State $R^\star(X)\gets$ the exact region from \cref{alg:watch}
\State Order all candidate spans contained in $R^\star(X)$ by decreasing $p_f$ and take the shortest prefix $A_0(X)$ with $U_Q(A_0(X)\mid X)\ge q_0$
\State $A(X)\gets A_0(X)$ after removing, from least to most probable, every span whose removal preserves $U_Q(\cdot\mid X)\ge q_0$
\State Order $A(X)$ before all remaining spans, order each group by decreasing $p_f$, and form prefixes $C_j(X)$ with utilities $u_j(X)$
\State Apply the calibration and prediction steps of \cref{alg:capture_calibration,alg:capture_prediction}, sampling one query uniformly from each calibration video and using $h$ as the success test
\end{algorithmic}
\end{algorithm*}

\paragraph{From the optimal region to an exact anchor.}
Assume every positive-length integer-endpoint span in $[0,T]$ is available and $\tau\ge1/2$.
Then \cref{alg:watch} solves \cref{eq:anchor} exactly.
We establish Assumption~\ref*{ass:oracle} by showing that region and span-set optimization have the same minimum watch duration.

\emph{From a span set to a watched region.}
Any span set $C$ gives $R(C)=\bigcup_{s\in C}s$ with $|R(C)|=W(C).$
Any selected span $s\in C$ matching $y$ also lies inside $R(C)$.
Thus span-set success implies region success,
\[
U_f(R(C)\mid x)\ge U_Q(C\mid x).
\]
The region therefore reaches the same threshold at equal duration, so the optimal region cannot be longer.

\emph{From a watched region to a span set.}
For any watched region $R$, select all candidates inside it,
\[
C_R=\{s\in\mathcal P:s\subseteq R\}.
\]
A matching clip for $y$ lies within one component $G$.
Step 1 of \cref{prop:dp} gives $|y\cap G|\ge\tau|y|$, so $y\cap G$ itself matches $y$.
Both $y$ and $G$ have integer endpoints, so their nonempty intersection belongs to the full pool and to $C_R$.
Conversely, every matching span selected by $C_R$ lies inside $R$.
The success rules therefore agree,
\[
U_Q(C_R\mid x)=U_f(R\mid x).
\]
All selected spans lie inside $R$, giving $W(C_R)\le |R|.$
The span set therefore reaches the same threshold with no greater duration.
Together, both directions establish equal minima in \cref{eq:oracle,eq:anchor}.

\emph{Constructing the anchor.}
For the exact region $R^\star(X)$ from \cref{alg:watch}, let $C_{R^\star}$ contain all pool spans inside it.
Since
\[
U_Q(C_{R^\star}\mid X)=U_f(R^\star(X)\mid X)\ge q_0
\]
adding those spans in decreasing model-probability order eventually reaches $q_0$.
Algorithm~\ref{alg:s:capture} calls the first qualifying prefix $A_0(X)$.
Its spans lie inside $R^\star(X)$, giving $W(A_0(X))\le |R^\star(X)|.$
Since $A_0(X)$ reaches the threshold, its duration equals the common optimum, solving \cref{eq:oracle} exactly.
Removing redundant spans preserves $U_Q(\cdot\mid X)\ge q_0$ and cannot increase duration.
Thus \cref{alg:s:capture} satisfies Assumption~\ref*{ass:oracle} and \cref{thm:watch} applies.

\paragraph{Long videos and the span cap.}
On long videos, we limit computation by retaining only the most probable spans.
Marginal coverage still holds if the fallback prediction at threshold 1 succeeds.
The watch-duration bound additionally requires an exact anchor over the pool defining $U_Q$.

On the three main benchmarks, all whole-second spans fit within the 12,000-span cap.
Their union is $[0,\lfloor T\rfloor]$, which covers the video when $T$ is an integer.
At threshold 1, Line~4 of \cref{alg:capture_prediction} returns all candidate subclips from the entire video, whose watched region is $[0,T]$.
It therefore succeeds under the region rule even when the ordinary pool omits a final partial second.
Span-set success under $a_\tau$ can fail for short annotations whose endpoints lie between grid points.
The best whole-second match for $[3.4,4.2]$, for example, has tIoU 0.5 and fails a request of 0.7.
If even the full-pool prediction can fail, \cref{thm:validity} gives $1-\alpha-p_0$, where $p_0$ is its failure probability under the chosen rule.

On long videos, we retain the 12,000 most probable spans per query and renormalize their probabilities (\cref{sec:supp:impl:scoring}).
This pool defines $Q$, the anchor and every prefix used when $\hat q<1$.
Calibration examples without a successful retained prefix receive score 1.
At threshold 1, prediction bypasses the cap and returns all candidate subclips from the entire video, preserving marginal coverage under the region rule.
If this uncapped prediction can fail, the guarantee is $1-\alpha-p_0$.
Here $p_0$ measures failure of the uncapped prediction, not failure of the retained pool.

For \cref{thm:watch}, define $Q$ over the retained pool, evaluate $e_+$ and $e_-$ against the true $P$, and require Assumption~\ref*{ass:model}.
Both the error definitions and $\mathrm{OPT}_P$ must use span sets from that pool.
The anchor must solve \cref{eq:oracle} exactly over it and then be made inclusion-minimal.
Capping can break this exactness because $U_f(R\mid X)$ counts candidates matched by any clip in $R$, including clips that were not retained.
If the region reaches $q_0$ but its retained spans do not, we increase the duration budget until they do.
This meets the threshold but need not minimize watch duration over retained spans.
Assumption~\ref*{ass:oracle} may therefore fail, so \cref{thm:watch} gives no oracle comparison for these runs.
Coverage still holds through the full-pool fallback as described above.

\FloatBarrier

\subsection{Why the oracle needs a higher success level}
\label{sec:supp:proofs:lower}

The upper bound compares \texttt{CAPTURE} with an oracle asked to succeed more often than the user requests.
Its success level is $q_0+\epsilon_L$.
Choosing the smallest $q_0$ allowed by \cref{eq:q0_condition}, with $q_0+\epsilon_L\le1$, gives $r_n$ in \cref{eq:coverage_relaxation}.
As the calibration sample grows, $r_n$ approaches $1-\alpha+\epsilon_A+\epsilon_L$ when $\log(1/\delta)=o(n)$.
We now show why the model-error terms remain necessary.
No uniformly valid method, conformal or otherwise, can generally remove them, even with arbitrarily many calibration examples.
The proof adapts impossibility results for conditional coverage~\cite{vovk2012conditional,lei2014distribution,barber2021limits}.

We consider realizable distribution--model pairs satisfying $\mathbb E\,e_+(X)\le\epsilon_A$ and $e_-(X)\le\epsilon_L$ almost surely under $P_X$.
These form the class $\mathfrak F_0(\epsilon_A,\epsilon_L)$ in \cref{thm:lb_minimax_sharpness}.
The errors $e_+$ and $e_-$ use the span-set rule (\cref{eq:overestimation_error,eq:underestimation_error}), with $\beta=0$.

A method uses $n$ calibration pairs $(X_i,Y_i)$, the model and test input $X$ to return a span set $\widehat C_n(X)$, possibly with randomization.
It must satisfy $\Pr\big(a_\tau(\widehat C_n(X),Y)=1\big)\ge1-\alpha$ for every pair in this class.
Let $\mathfrak A_n$ contain all methods satisfying this requirement.
The worst-case distribution may vary with calibration size.
We select $M_n$ equally likely identifiers from an infinite input space, with $M_n/n\to\infty$, so the test identifier is absent from calibration with probability approaching one.
All videos have duration $T$, and all integer-endpoint spans in $[0,T]$ are candidates.

\begin{restatedtheorem}{thm:lb_minimax_sharpness}[Minimax sharpness of coverage relaxation]
Fix $\tau,\alpha\in(0,1)$ and
$\epsilon_A,\epsilon_L\ge0$ with
$\epsilon_A+\epsilon_L<\alpha$. Define
\begin{equation}
r^\star=1-\alpha+\epsilon_A+\epsilon_L.
\tag{\ref*{eq:critical_level}}
\end{equation}
There exist a sufficiently large fixed temporal
grid length $T$ and a constant $K_0>1$ such that,
for every fixed $r\in(0,r^\star)$, there is a
constant $c_r>0$, independent of $n$, satisfying
\begin{equation}
\begin{aligned}
&\liminf_{n\to\infty}
\inf_{\mathcal A_n\in\mathfrak A_n}
\sup_{(P,Q)\in\mathfrak F_0}
\\
&\quad\Pr\left(
\frac{W(\widehat C_n(X))}
{\operatorname{OPT}_P(X,r)}
\ge K
\right)\ge c_r
\end{aligned}
\tag{\ref*{eq:minimax_lower_bound}}
\end{equation}
for every $K\in(1,K_0]$. The conclusion also
holds for any sequence $K_n>1$ with $K_n\to1$.
The hard instances can be chosen with both
$P(Y\mid X=x)$ and $Q(\cdot\mid x)$ varying
nontrivially with $x$.
\end{restatedtheorem}

The following proposition gives the bound for all sufficiently large calibration samples, implying Theorem~2.


\begin{proposition}[Lower bound]
\label{prop:s:lower}
Let $\tau\in(0,1)$ and $\alpha\in(0,1)$, and let $\epsilon_A,\epsilon_L\ge0$ satisfy $\epsilon_A+\epsilon_L<\alpha$.
Set $r^\star=1-\alpha+\epsilon_A+\epsilon_L$.
Then there are a video duration $T$ and a factor $K_0>1$ with the following property.
For each oracle success level $r\in(0,r^\star)$, there exist constants $c_r>0$ and $N_r$, both independent of the method, such that the following holds.
For every $n\ge N_r$ and every method with marginal coverage at least $1-\alpha$ uniformly over $\mathfrak F_0(\epsilon_A,\epsilon_L)$, there is a pair in this class for which
\[
\Pr\big(W(\widehat C_n(X))\ge K_0\,\mathrm{OPT}_P(X,r)\big)\ge c_r.
\]
The probability is over the calibration sample, test pair and any method randomness.
The pair can be chosen with both $P(Y\mid X=x)$ and $Q(\cdot\mid x)$ varying with $x$.
\end{proposition}

\begin{proof}[Proof of Theorem~2 from \cref{prop:s:lower}]
Fix $r\in(0,r^\star)$ and take $T$, $K_0$, $c_r$ and $N_r$ from \cref{prop:s:lower}.
For each $n\ge N_r$, any method in $\mathfrak A_n$ has a pair in $\mathfrak F_0(\epsilon_A,\epsilon_L)$ on which the probability is at least $c_r$.
Because $c_r$ and $N_r$ do not depend on the method, the infimum over $\mathfrak A_n$ of the worst-case probability is at least $c_r$ for all $n\ge N_r$.
The limit inferior is therefore at least $c_r$.
For $K\in(1,K_0]$, $W(\widehat C_n(X))\ge K_0\mathrm{OPT}_P(X,r)$ implies $W(\widehat C_n(X))\ge K\mathrm{OPT}_P(X,r)$.
This also covers any sequence $K_n>1$ with $K_n\to1$, since eventually $K_n\le K_0$.
\end{proof}

To prove \cref{prop:s:lower}, we construct inputs for which the oracle can safely return a short region but the method cannot tell when this is sufficient.
A short span matches only an inner moment, whereas a longer span matches both the inner moment and an outer one.
Each input belongs to an observable group that determines the model probabilities.
It also has a hidden type, called good or bad.
On good inputs, the true probability of the inner moment is higher than the model predicts, and on bad inputs it is lower.
Either difference may be zero.
The short prediction meets the oracle request $r$ on good inputs.
Because the method cannot identify the hidden type of an unseen input, it must watch longer on some good inputs to maintain marginal coverage.

\begin{proof}
\emph{Step 1. Choose two moments that require different watch durations.}
We construct an outer moment $y_0$ and an inner moment $y_1$ whose shortest matches require $\ell_0>\ell_1$ seconds.
Every match to $y_0$ will also match $y_1$, giving duration ratio $K_0=\ell_0/\ell_1$.
Choose an integer $g\ge1$ so that $T=\lfloor g/\tau\rfloor+1$ satisfies $T(1-\tau)\ge2$.
Set $y_0=[0,T]$, $y_1=[1,T-1]$, $\ell_0=g+1$ and $\ell_1=\lceil\tau(T-2)\rceil$.
The inner moment removes one second from each end of the outer one.

From $g/\tau<T\le g/\tau+1$ and $\tau<1$, we get $g<\tau T\le g+\tau<g+1$ and hence $\ell_0=g+1=\lceil\tau T\rceil$.
Every $s\subseteq[0,T]$ satisfies $\operatorname{tIoU}(s,y_0)=|s|/T$ because $y_0$ contains it.
Matching $y_0$ therefore requires exactly $|s|\ge\tau T$, or $|s|\ge\ell_0$ for integer-length spans.
Such a span also matches $y_1$, as three cases show.

If $s\subseteq y_1$, then $\operatorname{tIoU}(s,y_1)=|s|/(T-2)$ exceeds $\tau$ because $|s|\ge\ell_0>\tau T>\tau(T-2)$.
If $s=y_0$, then $\operatorname{tIoU}(s,y_1)=(T-2)/T$, and $T(1-\tau)\ge2$ gives $(T-2)/T\ge\tau$.
Otherwise, integer endpoints mean that $s$ contains exactly one outer second, $[0,1]$ or $[T-1,T]$.
In the first case, $s=[0,e]$ with $\ell_0\le e\le T-1$.
Its intersection and union with $y_1$ have lengths $e-1$ and $T-1$.
Since $e\ge\ell_0=g+1$, we have $e-1\ge g$, while $\tau(T-1)=\tau T-\tau\le g$.
Thus $\operatorname{tIoU}(s,y_1)=(e-1)/(T-1)\ge g/(T-1)\ge\tau$.
The case where the span includes the last outer second is symmetric.

Now choose an integer-endpoint span $D\subseteq y_1$ with $|D|=\ell_1$.
Since $\ell_1=\lceil\tau(T-2)\rceil$, it matches $y_1$ with $\operatorname{tIoU}(D,y_1)=\frac{\ell_1}{T-2}\ge\tau$.
But $\tau(T-2)\le\tau T-\tau\le g$ gives $\ell_1\le g<\ell_0$, so $D$ cannot match $y_0$.
No shorter span matches $y_1$.
The bound $\operatorname{tIoU}(s,y_1)\le |s|/(T-2)$ means that reaching tIoU $\tau$ requires $|s|\ge\tau(T-2)$ and hence $|s|\ge\ell_1$.

For a set $C$, let $\chi_1(C)$ and $\chi_0(C)$ indicate success on $y_1$ and $y_0$.
The matching relation gives $\chi_0(C)\le\chi_1(C)$.
If $W(C)<\ell_0$, every selected span is too short to match $y_0$, so success is possible only on $y_1$.
Any successful prediction needs at least $\ell_1$ seconds.
Set $K_0=\ell_0/\ell_1>1$.

\emph{Step 2. Define the model and true distributions.}
Fix $r<r^\star$.
We choose probabilities so that a short prediction meets the oracle's request on good inputs but falls below $1-\alpha$ when the type is unknown.
Each identifier's group $\sigma\in\{1,2\}$ determines $Q$, while its hidden type determines the difference between $P$ and $Q$.
In either group, an input is good with probability $\omega\in(0,1)$.
We choose a rational value so that a finite collection can contain exactly this proportion of good inputs.
Two distinct positive values $\theta_1,\theta_2$ distinguish the groups' model probabilities.
They will determine how far success on unseen inputs falls below the request in Step 4.

Let $\kappa_\sigma$ be the model probability of $y_1$.
On bad inputs, the model overestimates this probability by $b$.
Bad inputs occur with probability $1-\omega$ and are the only inputs on which success is overestimated.
Setting $b=\epsilon_A/(1-\omega)$ makes average overestimation equal to $\epsilon_A$.
Set $\kappa_\sigma=1-\alpha+\epsilon_A-\omega\epsilon_L-\theta_\sigma$.
The model assigns $\kappa_\sigma$ to $y_1$ and $1-\kappa_\sigma$ to $y_0$.
The true probability of $y_1$ is $\kappa_\sigma+\epsilon_L$ on good inputs and $\kappa_\sigma-b$ on bad inputs, with the remainder assigned to $y_0$.
Either difference may be zero when its error allowance is zero.

Choose sufficiently small rational $\omega\in(0,1)$ and distinct $\theta_1,\theta_2>0$ satisfying, for each $\sigma\in\{1,2\}$,
\[
\omega\epsilon_L+\theta_\sigma<r^\star-r
\quad\text{and}\quad
1-\alpha-\theta_\sigma-\omega\epsilon_L-\frac{\omega\epsilon_A}{1-\omega}>0.
\]
The first condition makes $\{D\}$ succeed with probability above $r$ on good inputs.
The second keeps the true probability of the inner moment positive on bad inputs.
Such choices exist because $r<r^\star$.
Choose $\omega>0$ with $\omega\epsilon_L<r^\star-r$, then distinct positive $\theta_\sigma<r^\star-r-\omega\epsilon_L$.
The second inequality holds for sufficiently small choices by continuity, since its left side is $1-\alpha>0$ at $\omega=\theta_\sigma=0$.

The probabilities are valid.
On good inputs, $\kappa_\sigma+\epsilon_L=r^\star-\omega\epsilon_L-\theta_\sigma<1$ because $r^\star<1$.
On bad inputs, the second condition gives $\kappa_\sigma-b>0$.
These bounds also give $\kappa_\sigma>0$ and $\kappa_\sigma<1$, so all model and true probabilities lie in $[0,1]$.
Use $M$ equally likely identifiers, with half assigned to each group and proportion $\omega$ good in each group.
Choose an even $M$ for which $\omega M/2$ is an integer.
In Step 4, we set $M=M_n$.

\emph{Step 3. Verify the model-error bounds and calculate the oracle duration.}
True and estimated success differ only when a prediction matches just one moment,
\[
U_P(C\mid X)-U_Q(C\mid X)
=\big(P(y_1\mid X)-\kappa_\sigma\big)
 \big(\chi_1(C)-\chi_0(C)\big).
\]
Since matching $y_0$ implies matching $y_1$, the second factor is in $\{0,1\}$ and is one exactly when only $y_1$ matches.
The difference is therefore zero or $\epsilon_L$ on good inputs and zero or $-b$ on bad inputs.
The set $\{D\}$ attains the differences $\epsilon_L$ on good inputs and $-b$ on bad inputs.
Thus good inputs have $e_-(X)=\epsilon_L$ and $e_+(X)=0$, while bad inputs have $e_-(X)=0$ and $e_+(X)=b$.
Thus $e_-(X)\le\epsilon_L$ everywhere and $\mathbb E\,e_+(X)=(1-\omega)b=\epsilon_A$.
Both moments belong to the pool and match themselves, so the pair is realizable and belongs to $\mathfrak F_0(\epsilon_A,\epsilon_L)$.

On good inputs, $\{D\}$ succeeds exactly on $y_1$, with probability
\[
U_P(\{D\}\mid X)
=\kappa_\sigma+\epsilon_L
=r^\star-\omega\epsilon_L-\theta_\sigma.
\]
By the first parameter condition, this probability exceeds $r$, so the oracle needs only $\ell_1$ seconds.
If $W(C)<\ell_1$, every selected span is too short to match either moment, giving zero success probability.
Hence $\mathrm{OPT}_P(X,r)=\ell_1$ on every good input.

\emph{Step 4. Marginal coverage forces long outputs on unseen inputs.}
We find an assignment that forces extra watching by first averaging over possible assignments.
In each group, choose the good identifiers uniformly among subsets of size $\omega M/2$, independently across groups, and set $M=M_n$.
The method must have coverage at least $1-\alpha$ for every fixed assignment, so it must also satisfy this requirement after averaging.
Unlike the oracle, it sees only the model and calibration data.

\emph{Step 4a. The hidden type of an unseen input remains uncertain.}
Let $E$ mean that the test identifier is absent from the $n$ calibration inputs.
Equal identifier probabilities give $\pi_n=\Pr(E)=(1-1/M_n)^n\to1$, using $M_n/n\to\infty$.
The model reveals the group but not the type.
Even revealing all calibration identifiers' types leaves uncertainty about the test identifier.

Since $M_n/n\to\infty$, take $n$ large enough that $M_n/2>n$.
Suppose calibration contains $d\le n$ distinct identifiers from the test identifier's group, of which $d_+$ are good.
Of its initial $M_n/2$ identifiers, $\omega M_n/2$ were good.
This leaves $\omega M_n/2-d_+$ good identifiers among the $M_n/2-d$ unseen ones.
Given the observed groups and types, calibration labels give no further information about unobserved types.
All remaining assignments are equally likely.
On $E$, the test identifier is therefore good with probability $\frac{\omega M_n/2-d_+}{M_n/2-d}$.
Its difference from $\omega$ is $\frac{\omega d-d_+}{M_n/2-d}$, whose absolute value is at most $\frac{d}{M_n/2-d}\le\frac{n}{M_n/2-n}$ because $0\le d_+\le d$.

The method does not observe calibration types.
Let $\omega'$ be the probability that the test identifier is good on $E$, given the calibration data, model and test input.
Averaging over possible calibration types preserves $|\omega'-\omega|\le\frac{n}{M_n/2-n}$.
The true probability of $y_1$ given the method's information on an unseen input in group $\sigma$ is therefore
\[
\omega'(\kappa_\sigma+\epsilon_L)
 +(1-\omega')(\kappa_\sigma-b)
=1-\alpha-\theta_\sigma
 +(\omega'-\omega)(\epsilon_L+b).
\]
As $|\omega'-\omega|\to0$, the correction $(\omega'-\omega)(\epsilon_L+b)$ vanishes.
For sufficiently large $n$, this probability is below $1-\alpha$, so short predictions, which can match only $y_1$, fall short of the request.

\emph{Step 4b. Make the uncertainty bounds uniform over observations.}
Let $\theta=\min\{\theta_1,\theta_2\}>0$ be the smaller group margin.
Choose $N_r$ so that, for all $n\ge N_r$, $M_n/2>n$ and four bounds hold for every possible observation.
First, unseen inputs remain common, $\pi_n\ge\frac12$.
Second, success on seen inputs alone cannot offset the shortfall on unseen inputs with short predictions,
\[
\pi_n(\alpha+\theta/2)\ge\alpha+\theta/4.
\]
Third, an unseen input still has a positive chance of being good, $\omega'\ge\frac{\omega}{2}$.
Fourth, short predictions remain insufficient in either group on $E$,
\[
\Pr(Y=y_1\mid\text{method's information},E,\sigma)
\le1-\alpha-\theta/2.
\]
These bounds eventually hold because $M_n/n\to\infty$ gives $\pi_n\to1$ and $n/(M_n/2-n)\to0$.
Thus $\omega'\to\omega$ uniformly over observations, and $\Pr(Y=y_1\mid\text{the method's information},E,\sigma)$ converges uniformly to $1-\alpha-\theta_\sigma\le1-\alpha-\theta$.
These requirements depend only on $n$, $M_n$ and the construction, making $N_r$ independent of the method.
Fix $n\ge N_r$.

\emph{Step 4c. Use marginal coverage to force long outputs.}
On $E$, watch duration below $\ell_0$ allows success only on $y_1$, with conditional probability at most $1-\alpha-\theta/2$ by Step 4b.
Write $\rho_n=\Pr\big(W(\widehat C_n(X))\ge\ell_0\mid E\big)$ for the chance of a long output on an unseen input.
To obtain an upper bound on success, count every seen input and every long output as successful.
Since the method guarantees coverage, even this upper bound must reach $1-\alpha$,
\begin{equation*}
\begin{aligned}
1-\alpha
&\le(1-\pi_n)
 +\pi_n\big[(1-\rho_n)(1-\alpha-\theta/2)+\rho_n\big]\\
&=1-\pi_n(1-\rho_n)(\alpha+\theta/2).
\end{aligned}
\end{equation*}
Rearranging gives $\rho_n\ge1-\frac{\alpha}{\pi_n(\alpha+\theta/2)}$.
The second bound in Step 4b then gives $\rho_n\ge\frac{\theta}{4\alpha+\theta}$, a positive lower bound independent of calibration size.

These long outputs cannot all be reserved for bad inputs.
Given the method's information on $E$, its output depends only on its own randomization, independently of the hidden test type.
The input remains good with probability at least $\omega/2$.
For any observation, the chance of both a good input and a long output is at least $\omega/2$ times the chance of a long output.
Averaging gives probability at least $\omega\rho_n/2$ conditional on $E$, or $\pi_n\frac{\omega\rho_n}{2}$ unconditionally.
Using $\pi_n\ge1/2$ and $\rho_n\ge\theta/(4\alpha+\theta)$,
\[
\pi_n\frac{\omega\rho_n}{2}
\ge
\frac{\omega\theta}{4(4\alpha+\theta)}
=:c_r.
\]
On good inputs $\mathrm{OPT}_P(X,r)=\ell_1$, so this event gives
\[
W(\widehat C_n(X))
\ge\ell_0
=K_0\,\mathrm{OPT}_P(X,r).
\]
For this method and calibration size $n$, at least one fixed assignment attains the average bound and supplies a pair in $\mathfrak F_0(\epsilon_A,\epsilon_L)$.
Since $\theta_1\ne\theta_2$, both $P(Y\mid X=x)$ and $Q(\cdot\mid x)$ vary across groups.
\end{proof}

The comparison factor is $K_0=\frac{\lceil\tau T\rceil}{\lceil\tau(T-2)\rceil}$, giving $K_0=1.5$ for $\tau=1/2$ and $T=5$.
This does not rule out a weaker watch-duration comparison with factor $1/\tau$.
Deriving such a bound from whole-moment containment requires a separate argument.
The construction allows more than one possible annotation for each input and uses enough inputs that the test identifier is unlikely to appear in calibration.

The region rule gives the same lower bound for outputs formed from integer-endpoint spans and the same oracle $\mathrm{OPT}_P$.
Their integer-valued watch duration means $W(\widehat C_n(X))<\ell_0=g+1$ permits at most $g<\tau T$ seconds.
Every contained clip is too short to match $y_0$, so the same argument forces long regions with positive probability on good inputs, whose oracle duration is $\ell_1$.
On these realizable instances, \cref{thm:validity} gives \texttt{CAPTURE} coverage at least $1-\alpha$ under either rule.
Here $r^\star$ is the asymptotic limit of $r_n$ in \cref{eq:coverage_relaxation}.
One query per video is a special case of video-level sampling, so the lower bound also applies with videos as calibration units.

\subsection{Containing a moment versus predicting a matching span}
\label{sec:supp:proofs:vacuous}

A watched region can contain the entire moment and still have low tIoU with it because the region includes unrelated footage.
For measurable sets $A,B\subseteq[0,T]$ with $|A\cup B|>0$, define $\operatorname{tIoU}(A,B)=\frac{|A\cap B|}{|A\cup B|}$.
Part (i) shows that no fixed prediction can match every possible contained moment when moments may be arbitrarily short.
Part (ii) separates missed footage from extra footage and shows how expanding the region affects each.

\begin{proposition}[Containment gives no positive tIoU bound]
\label{prop:s:vacuous}
Suppose that $R\subseteq[0,T]$ is a measurable region that contains an interval of positive length.
Let $\mathcal I_T$ be the intervals of positive length in $[0,T]$.
\textup{(i)} For every fixed measurable prediction $s\subseteq[0,T]$, the tIoU with a positive-length moment $y\subseteq R$ can be arbitrarily close to zero,
\[
\inf\{\operatorname{tIoU}(s,y):y\in\mathcal I_T,\ y\subseteq R\}=0.
\]
\textup{(ii)} For any moment $y$, the tIoU loss is the sum of the unwatched part of the moment and the watched footage outside it, each normalized by the union duration,
\begin{equation}
1-\operatorname{tIoU}(R,y)=\frac{|y\setminus R|}{|R\cup y|}+\frac{|R\setminus y|}{|R\cup y|}.
\label{eq:s:split}
\end{equation}
As $R$ grows under set inclusion, the first term cannot increase and the second cannot decrease.
\end{proposition}

For $s=R$, an arbitrarily short contained moment $y\subseteq R$ leaves most watched footage outside it, driving tIoU to zero.
For other fixed $s$, $|s\cap y|\le|y|$ gives the same conclusion.
Containment ensures that a matching clip exists, without making one fixed prediction match every contained moment.

\begin{proof}
(i) If $|s|=0$, then $|s\cap y|=0$ for every positive-length $y$, giving tIoU zero.
Otherwise $|s|>0$, and the assumed interval $[t_1,t_2]\subseteq R$ has $t_2>t_1$.
For each positive-length $y\subseteq[t_1,t_2]$, we have $|s\cap y|\le|y|$ and $|s\cup y|\ge|s|$, so
\[
\operatorname{tIoU}(s,y)
=\frac{|s\cap y|}{|s\cup y|}
\le\frac{|y|}{|s|}.
\]
Choosing subintervals of $[t_1,t_2]$ with positive lengths approaching zero gives $|y|/|s|\to0$.
Their tIoU approaches zero, and nonnegativity makes the infimum zero.

(ii) The union $R\cup y$ splits into disjoint overlap $R\cap y$, extra footage $R\setminus y$ and missed footage $y\setminus R$.
Thus $|R\cup y|-|R\cap y|=|R\setminus y|+|y\setminus R|$.
Using $1-\operatorname{tIoU}(R,y)=(|R\cup y|-|R\cap y|)/|R\cup y|$ and dividing by $|R\cup y|>0$ gives \cref{eq:s:split}.
As $R$ grows under inclusion with $y$ fixed, $|y\setminus R|$ cannot increase and $|R\cup y|$ cannot decrease, so the first term cannot increase.
For the second, the disjoint union of $R\setminus y$ and $y$ gives
\[
\frac{|R\setminus y|}{|R\cup y|}
=
\frac{|R\setminus y|}
     {|R\setminus y|+|y|}.
\]
Here $|R\setminus y|$ cannot decrease and $|y|$ is fixed.
Since $z\mapsto z/(z+|y|)$ is nondecreasing for $z\ge0$ whenever $z+|y|>0$, the second term cannot decrease.
\end{proof}
