# Supplementary material for: CAPTURE: Minimizing Watch Time for Reliable Temporal Video Grounding
Source: arXiv:2611.38466 source file (2026-11-28)
Supplement: Supplementary file 6 [file results.tex]

\section{Additional \texttt{CAPTURE} results}
\label{sec:supp:results}

\texttt{CAPTURE} can reduce watch duration in two ways.
It asks for one matching clip rather than the whole moment, and it chooses where to watch using the span probabilities.
We examine both contributions, region quality, calibration and model errors relevant to the watch-duration bound.
\Cref{tab:supp:methods} extends the main comparison, and \cref{fig:watch-distribution} shows variation across queries.
Watch denotes normalized watch duration $W(C)/T$.
Reported success rates are empirical test averages.
Marginal coverage averages over calibration and test sampling, so an individual split or subgroup need not meet the request.
\supptab{set_methods_full}
\supppinnedfig{fig/watch-distribution}{3}

\subsection{Comparison with prior work}
\label{sec:supp:results:fair}

\input{fig/supp/qualitative-success}

\paragraph{Separating the target from the construction.}
Prior conformal grounding, COVER~\cite{mohamed2026cover}, widens one answer to contain the whole moment, or the temporal hull of multiple annotations.
This meets our matching-clip criterion at any tIoU but can require more footage than one sufficiently accurate clip.
The main-paper configuration watches less in all 108 cells of \cref{tab:main}, watching an average 43.1\% of the video versus 66.1\%.
We explain the gap by first requiring both methods to contain a whole moment, then recalibrating the prior method for one matching clip.

\paragraph{Requiring whole-moment containment.}
At $\tau=1$, we clip annotations at $\lfloor T\rfloor$ for every method.
This shortens 578 of 3,720 Charades-STA moments and 1,413 of 5,675 ActivityNet Captions moments by at most one second.
With the exact anchor, \texttt{CAPTURE} watches more than COVER at 70\% requested success (\cref{tab:supp:tau1}).
Mean watch duration at 70\%, 80\% and 95\% success is 56\%, 63\% and 80\% of the video, versus 53\%, 65\% and 90\%.
The calibrated greedy answer watches least at 70\% and 80\%, requiring 51\% and 62\% of the video.
At 80\%, the saving falls from 28\% of the video at tIoU 0.5 to 2\% at tIoU 1.
Much of the original reduction therefore comes from the matching-clip target.
The selected QVHighlights examples in \cref{fig:supp:qualitative-success,fig:supp:qualitative-failure} use TimeLens2-8B at tIoU 0.5 and 80\% requested success.
They illustrate the fit-selected configuration and COVER at median calibrated thresholds over 1,000 splits.

\supptab{set_tau1}

\paragraph{When the most probable span misses.}
We identify peaks by repeatedly selecting the most probable remaining span and removing those overlapping it at tIoU $\ge0.5$.
In a wrong-peak query, the most probable span misses but a later selected span contains a matching clip.
Spans overlapping it at tIoU $\ge0.5$ must together carry at least 5\% of model probability.
Such queries account for 10\% to 30\% of each model--benchmark pair, averaging 16\%.
At $\tau=1$ and 80\% requested success, COVER succeeds on 72\% of these queries and 85\% of the rest, compared with 90\% and 78\% for \texttt{CAPTURE}.
Widening enough to reach another peak also enlarges answers on easier queries.
\texttt{CAPTURE} can instead keep separate segments and skip the gap.

Whole-moment containment must reach both annotated boundaries despite the model's uncertainty about them.
For TimeLens2-8B on Charades-STA, 32\% of the remaining queries require spans holding at least 0.99 of total model probability before a probability-ordered prefix contains the whole moment.

For matched empirical success, we choose thresholds from test annotations within each query group.
This diagnostic cannot be deployed.
With the exact anchor, \texttt{CAPTURE} ties COVER on wrong-peak queries at 70\% and watches less at higher rates, whereas COVER watches less on the remaining queries up to 85\% (\cref{tab:supp:tau1}).
Changing span order saves at most 1\% of the video across requests and query groups, and sharpening the probabilities does not help on the remaining queries.

\paragraph{Calibrating COVER for one matching clip.}
We recalibrate COVER's scaling rule for one matching clip.
For answer length $\ell=\hat e-\hat s$ and $\mu\ge-1/2$, the region is $[\hat s-\mu\ell,\hat e+\mu\ell]\cap[0,T]$.
A query's score is the smallest $\mu$ whose region contains a matching clip at tIoU $\tau$.
The scale is the $k_n$-th smallest score from one uniformly sampled query per calibration video.
This gives the marginal guarantee in \cref{thm:validity}, but lacks the exact anchor required for the watch-duration bound.
The calibrated greedy answer instead uses a discrete scale grid.

Retargeting lowers mean watch duration at tIoU 0.5 and 80\% from 64.6\% to 41.6\% of the video, versus 37.1\% for \texttt{CAPTURE} (\cref{tab:supp:retarget}).
Across 108 cells, the main-paper configuration of \texttt{CAPTURE} averages 43.1\% of the video versus 48.2\%, an 11\% reduction, and watches less in 86.
Mean watch duration falls by 3\%--17\% at each request.
Calibrating on all queries changes normalized watch duration by at most 0.008 but loses the video-level guarantee.
The target explains most of the gap, with a further reduction from region construction.
\supptab{set_retarget}

\subsection{Region construction, localization and calibration}
\label{sec:supp:results:regions}
\label{sec:supp:results:calibration}

\paragraph{Choosing the watched region.}
\Cref{tab:supp:watch} compares region constructions using the same span probabilities and calibration procedure.
At 80\% requested success, the exact anchor with continuation watches least or ties in only 1 of 18 cells, or 3 when ties at two decimals count, as in the bold marks.
Enumerate-and-cover saves 0.1\%--2.2\% of the video in 13 cells, the gain-per-second anchor saves 0.2\%--0.9\% in 6, and per-second thresholding saves 0.1\%--3.1\% in 7.
The exact anchor minimizes watch duration at a fixed model-estimated success threshold.
Calibration can choose different thresholds for each family, so the shortest anchor need not give the shortest final prediction.
\supptab{set_watch}

Without continuation, watch duration changes by less than 0.1\% of the video in 13 of 18 cells and increases by 0.4\% to 1.9\% in the other 5.
Optimizing regions independently at each threshold can move the region to another probability peak as the threshold increases, losing a previously matched moment.
These regions need not be nested, so our marginal guarantee does not apply.
Mean success falls more than 0.002 below the request in 45 of 108 cells, so we exclude this construction.

\paragraph{What the viewer receives.}
At tIoU 0.5 and 80\% success, \texttt{CAPTURE} has higher precision than the prior method in all 18 model--benchmark pairs and than the calibrated greedy answer in 15 (\cref{tab:supp:quality}).
On QVHighlights, mean precision is 0.71, versus 0.35 and 0.66.
Its region contains a complete moment on only 23\% of queries, versus 90\% and 45\%, because a matching clip need not cover the whole moment.
The greedy answer has higher precision, 0.74, but succeeds on only 78\% of queries.
Per-second thresholding raises region tIoU from 0.48 to 0.59 but requires 28\% of the video instead of 24\%.
\supptab{set_quality}

A second grounding pass need not find the matching clip.
TimeLens2-8B regions contain a matching clip at tIoU 0.5 on 81\% of QVHighlights queries.
Rerunning the model on the returned footage succeeds on only 64\% of queries, versus 72\% on the whole video.
The guarantee concerns footage available to a viewer.
It does not ensure that another model pass succeeds or that every query is covered (\cref{fig:supp:qualitative-failure}).

\input{fig/supp/qualitative-failure}

\paragraph{Calibration units and data size.}
Treating all queries as exchangeable ignores related errors within a video.
This gives mean success more than 0.002 below the request in 22 of 72 cells, with a worst shortfall of 0.013 (\cref{tab:supp:units}).
Sampling one query per video lowers the worst shortfall to about 0.001 and meets \cref{thm:validity}'s assumptions.
With a tenth of the calibration videos, no trial triggers whole-video fallback at tIoU 0.5 and 80\%, but watch duration increases by up to 11\% of the video length (\cref{tab:supp:calsize}).
Fewer calibration videos increase $k_n/n$ and make the selected threshold more variable.
\supptab{set_units}
\supptab{set_calsize}

In all 18 cells, normalized watch duration differs by at most 0.01 between the fit-selected and best fixed $q_0$.
Coverage averages over moment lengths and need not hold within each length group.
Success across length bins ranges from 73\% to 91\% at tIoU 0.5 and an 80\% request.
At tIoU 0.7 and a 70\% request, success on moments longer than 30 seconds reaches only 64\% to 69\%.

\paragraph{Equal labeled-video budgets.}
To equalize labeled-video budgets, fixed-family baselines calibrate on both fit and calibration videos.
The exact anchor with continuation fixes $q_0=0.99$ without using calibration data to select it.
\texttt{CAPTURE} and the positional prior keep their existing fit procedures.
Mean watch duration is 43.1\% of the video for \texttt{CAPTURE}, 42.9\% for per-second thresholding, 42.7\% for enumerate-and-cover and 43.5\% for the exact anchor with continuation.
The calibrated greedy answer, calibrated MBR answer and COVER watch 49.0\%, 46.0\% and 65.1\% of the video.
Fit-video selection is close to the best fixed type in mean watch duration, but does not always win.

\subsection{Applicability of the watch-duration bound}
\label{sec:supp:results:bound}

\label{sec:supp:bound:practice}
\paragraph{How much model error the bound permits.}
The watch-duration theorem compares duration with an oracle when model errors are sufficiently small.
We test these sufficient conditions below.
Marginal coverage holds even when they fail.
\Cref{thm:watch} requires $q_0$ to satisfy \cref{eq:q0_condition}.
For $n=400$ and $\delta=0.1$, the rank gap $k_n/n-(1-\alpha)$ and the square-root term add 0.056 to the required success level.
The lower bound on $q_0$ is therefore $1-\alpha+0.056+\epsilon_A$.
Together with $q_0+\epsilon_L\le1$, this requires $\epsilon_A+\epsilon_L\le\alpha-0.056$.
The combined error can therefore be at most 0.144 at an 80\% request or 0.244 at 70\%.
With our 133 to 374 calibration videos, these terms add 0.06 to 0.11.
At an 80\% request, the combined error must then stay below 0.09, 0.14 and 0.12 for the 133, 374 and 233 calibration videos of QVHighlights, Charades-STA and ActivityNet Captions.

The theorem also requires an exact anchor, which fit-video selection chooses in 20 of 72 cells at 70\% and 80\% success.
If we restrict selection to the exact-anchor family with continuation, it chooses $q_0\ge0.99$ in 65 cells.
This leaves at most 0.01 for $\epsilon_L$.
Capping $q_0$ at 0.9 or 0.8 raises mean watch duration from 37.6\% of the video to 40.0\% or 40.5\%.
We therefore choose settings to minimize watch duration on fit videos, without imposing these sufficient conditions.

\paragraph{Measuring overestimation from anchor success.}
The definition of $e_+(X)$ gives $U_P(A(X)\mid X)\ge q_0-e_+(X)$ for anchor $A(X)$.
Let $H$ indicate whether the anchor's region contains a matching clip.
Any selected span counted as a match by $U_P$ makes this region successful.
Thus $\mathbb E H\ge q_0-\mathbb E e_+(X)$, or $\mathbb E e_+(X)\ge q_0-\mathbb E H$.
Up to sampling error, any valid upper bound $\epsilon_A$ must be at least the gap between $q_0$ and empirical anchor success.
Before calibration, anchors succeed less often than their threshold $q_0$ predicts in all 72 settings of \cref{tab:main} at 70\% and 80\% requests.
For TimeLens-8B on ActivityNet Captions at tIoU 0.5 and 80\%, anchor success is 74\% despite $q_0=0.995$, requiring $\epsilon_A\ge0.25$.

\paragraph{What the model-error conditions require.}
If each input has one fixed annotation, $U_P(C\mid X)$ is 0 or 1.
If $c^\star(X)\in\mathcal P$ is a shortest matching span on our temporal grid, then $\mathrm{OPT}_P(X,r)=|c^\star(X)|$ for $r\in(0,1)$ and $e_-(X)\ge1-U_f(c^\star(X)\mid X)$.
Hence $e_-(X)\le\epsilon_L<1-q_0$ implies $U_f(c^\star(X)\mid X)>q_0$ and $W(A(X))\le|c^\star(X)|$.
This condition requires high model-estimated success probability for a shortest matching candidate span.

\paragraph{Allowing uncertainty in the annotation.}
Charades-TimeLens provides a second annotation for 867 unchanged Charades-STA queries~\cite{zhang2025timelens}.
The annotation pairs have median tIoU 0.40, with 37\% reaching 0.5.
Since $U_P$ is linear in the conditional annotation distribution, we estimate it by weighting the two annotations equally.
At $q_0=0.99$, TimeLens2-8B and Qwen3-VL-8B still overestimate anchor success, averaged over the two annotations, by 0.09 to 0.16.
At $q_0\ge0.99$, at most 1.3\% of inputs satisfy $e_-(X)\le1-q_0$.
This condition requires, in particular, model-estimated success of at least $q_0$ for a region containing a matching clip for each annotation.

Even with annotation uncertainty, these models do not satisfy the theorem's sufficient conditions.
An anchor can nevertheless be as short as the oracle on individual inputs.
Across this two-annotation analysis, the anchor is no longer than the shortest region containing a matching clip for each annotation on 27\% to 69\% of inputs.
The theorem identifies a model property sufficient for short regions, but does not predict watch duration in these experiments.

\subsection{Span scoring}
\label{sec:supp:results:distribution}
\label{sec:exp:structure}

\paragraph{Trading computation for watch duration.}
Token trees score all spans from one cached video encoding (\cref{sec:supp:impl:scoring}).
On QVHighlights, TimeLens2-8B's exact scoring costs about 6.5 more GPU seconds per query than greedy decoding. \texttt{CAPTURE} saves about 55 seconds of viewing in a 150-second video compared with the prior method.
Long-video scoring costs motivate the approximations in \cref{sec:supp:impl:factorized}.

Spans overlapping the most probable span at tIoU $\ge0.5$ hold a median 0.78 to 0.96 of the normalized probability for TimeLens and Qwen3-VL, versus 0.39 to 0.68 for MiMo-VL-7B.
For TimeLens and Qwen3-VL, start--end mutual information divided by end entropy is at most 0.058.
Consistent with this weak dependence, multiplying exact endpoint marginals changes normalized watch duration by only $-0.017$ to $+0.015$ (\cref{tab:supp:fact}).
Computing these marginals still requires the exact joint distribution.
A separate end prompt avoids this cost but increases normalized watch duration by 0.03--0.07 for TimeLens2-8B.
The learned correction reduces median weighted total-variation distance from 0.33--0.41 to 0.14--0.20.
Across tIoU 0.5 and 0.7 at 70\% and 80\% success, it removes 86\% of the two-prompt product's extra watch duration on QVHighlights and 93\% on ActivityNet Captions.
On Charades-STA, watch duration is 37.6\% of the video versus 38.5\% with exact scoring. Success differs by less than 0.001 at each request.
This requires no extra grounder passes (\cref{fig:supp:twoprompt}).
For Charades-STA-Long, training on joined videos helps it handle the longer inputs.

\supptab{set_fact}

\section{Long videos and generalization}
\label{sec:supp:generalization}

\subsection{Multiple moments and longer videos}
\label{sec:supp:results:long}

\paragraph{Matching one of several moments.}
\label{sec:supp:hull}
\hypertarget{section*.38}{}%
Following QVHighlights~\cite{lei2021qvhighlights}, success requires a match to any annotated moment.
Prior conformal grounding targets their temporal hull~\cite{mohamed2026cover}.
Our guarantee concerns one matching clip, not recovery of every moment.

\paragraph{Charades-STA-Long.}
We concatenate 1,334 Charades-STA videos into 66 longer videos, each containing 17 to 22 source videos and lasting 554 to 627 seconds.
Annotations shift by their source video's starting time in the joined video.
Annotated moments occupy a median 1.2\% of the joined video's duration.
TimeLens2-8B scores up to 40 random queries per video, totaling 2,638.
The 20 fit videos contain only sources assigned to fitting.
Each trial divides the remaining videos into 18 calibration and 28 test videos.
Exact scoring retains 12,000 spans, holding median probability 0.997 and minimum 0.87.
The 768-frame cap gives 1.2 to 1.4 frames per second.

At tIoU 0.5, the exact anchor with continuation watches 9\%, 27\%, 45\% and 74\% of the video for requests of 50\%, 70\%, 80\% and 90\% (\cref{tab:supp:chlong}).
The calibrated greedy answer watches 23\% and 58\% of the video at the first two requests, then returns the whole video in 18\% of trials at 80\%.
Both calibrated single-answer baselines do so in most trials at 90\%.
\supptab{set_chlong}

Joining videos can introduce an unannotated occurrence of the queried action.
For 842 queries, another source video has a query with the same verb and object.
Among the 55 queries whose text appears in another source video, greedy predicts a span in that other source for 35\% and in the annotated source for 24\%.
Greedy predicts a span outside the annotated source video on 51\% of the remaining 1,796 queries.
Excluding these 842 queries lowers the exact anchor's watch duration by 0.6\%--3.1\% of the video, and it still watches less than calibrated single answers.
This annotation-based filter cannot be used at deployment.

With 18 calibration videos, requests of 50\%, 60\%, 70\%, 80\% and 90\% give mean success of 53\%, 64\%, 74\%, 84\% and 95\%, close to $k_n/19$.
At $\delta=0.1$, the rank and Hoeffding terms in \cref{eq:q0_condition} add 0.31--0.34 above the 50\%--80\% requests.
No $q_0<1$ satisfies the sufficient watch-duration condition at 70\% or higher.
Calibration can avoid the whole-video fallback for requested success up to $18/19$.
Higher requests require returning the entire video.
With thresholds chosen from test annotations, the exact anchor with continuation watches 6\%--36\% of the video at 50\%--80\% requests and 55\% at 90\%.
This non-deployable diagnostic shows that limited calibration data increases watch duration alongside model error and incomplete annotations.

\supptab{set_newpools}

\paragraph{Learning from longer videos.}
We train four Charades-STA-Long correction networks on the main benchmarks and three quarters of the joined fit videos.
Training excludes all calibration and test videos and their sources.
They remove 93\%--98\% of the two-prompt product's extra watch duration at 50\%--60\% requests and at least 87\% at 70\%--80\%, averaging 95\% overall and 96\% after filtering repeated actions.

\subsection{New benchmarks and model sizes}
\label{sec:supp:results:generalization}

\paragraph{Fixing the pipeline before evaluation.}
We fixed code, settings and evaluation claims on 2026-11-08 before testing 3,363 queries on 1,313 Charades-TimeLens videos and 2,056 queries on 623 ActivityNet-TimeLens videos~\cite{zhang2025timelens}.
The former re-annotates Charades-STA, while the latter uses videos outside our ActivityNet Captions pool.
Across 1,000 trials, \texttt{CAPTURE} watches less than the prior method and calibrated greedy answer at all six requests (\cref{tab:supp:newpools}).
Mean success ranges from 0.00001 below to 0.007 above the request across 18 cells.

All three model--benchmark pairs satisfy three claims fixed before evaluation.
\texttt{CAPTURE} watches less than the prior method at all six requests and the calibrated greedy answer at five or more. Its normalized watch duration is within 0.01 of the best fixed region type at four or more.
A fourth claim, written for a Learn then Test variant, predicted test success below the request in at most 10\% of trials.
It does not hold for the split-conformal procedure.
Among trials without whole-video fallback, about half fall below the request.
The marginal guarantee averages success over calibration and test sampling and does not imply this bound across trials.

We reuse span probabilities for the 867 Charades-TimeLens queries whose text is unchanged.
Resolving near ties differently in a separate greedy decoding run changes answers on 6\% of TimeLens2-8B and 33\% of Qwen3-VL-8B queries, affecting only the baselines.
ActivityNet-TimeLens moments occupy a median 3.5\% of video duration, versus 27.5\% on ActivityNet Captions.
Videos last 150--267 seconds.
The cap removes spans on 1,963 of 2,056 queries while retaining a median 0.99999 and minimum 0.885 of total probability.

\supptab{set_size}

\paragraph{Model size.}
Seven Qwen3-VL and TimeLens2 models from 2B to 32B give 126 cells.
\Cref{tab:supp:size} shows two of six requests over 1,000 trials.
\texttt{CAPTURE} watches less than COVER in all 126 cells and the calibrated greedy answer in 125, saving an average 10\% of the video against the latter.
The exception is TimeLens2-8B on Charades-STA at tIoU 0.7 and 70\%, where it watches an additional 0.4\% of the video.
These counts use fit-video selection of the region type.
With the main-paper exact anchor, the counts are 126 and 120.
Mean success is never more than 0.001 below a request.
Qwen3-VL-32B watches least in 17 of its 18 cells and Qwen3-VL-2B most in 15.
Duration decreases strictly with size in 12 of 18 Qwen3-VL cells and 10 of 18 TimeLens2 cells.
Larger models usually need less viewing, although 4B and 8B models sometimes exchange rank.
