# Supplementary material for: CAPTURE: Minimizing Watch Time for Reliable Temporal Video Grounding
Source: arXiv:2611.38466 source file (2026-11-28)
Supplement: Supplementary file 7 [file set_calsize.tex]

\begin{table}[!tbp]
\caption{\textbf{Fewer calibration videos increase watch duration while preserving marginal coverage.}
\texttt{CAPTURE} uses the main-paper configuration, with $q_0$ fixed at its validation choice and only the number of calibration videos changed.
At tIoU\,$\ge$\,0.5 and 80\% requested success, each of 1,000 trials randomly subsamples its calibration videos.
Cal. follows \cref{tab:supp:methods}.
Full sets contain 133, 374 and 233 videos on QVHighlights, Charades-STA and ActivityNet Captions.
With a tenth of the calibration videos, mean success is at least 0.81 in all 18 model--benchmark pairs.
Watch is shown to three decimals.}
\label{tab:supp:calsize}
\hypertarget{table.caption.103}{}%
\centering
\scriptsize
\setlength{\tabcolsep}{0.95pt}
\begin{adjustbox}{max width=\columnwidth}
\begin{tabular}{@{}ll cc cc cc cc@{}}
\toprule
& & \multicolumn{2}{c}{10\%} & \multicolumn{2}{c}{25\%} & \multicolumn{2}{c}{50\%} & \multicolumn{2}{c}{100\%} \\
\cmidrule(lr){3-4}\cmidrule(lr){5-6}\cmidrule(lr){7-8}\cmidrule(lr){9-10}
\textbf{Benchmark} & \textbf{Model} & Cal. & Watch & Cal. & Watch & Cal. & Watch & Cal. & Watch \\
\midrule
Charades-STA & Qwen3-VL-4B & \cmark & 0.380 & \cmark & 0.352 & \cmark & 0.349 & \cmark & 0.343 \\
 & Qwen3-VL-8B & \cmark & 0.349 & \cmark & 0.329 & \cmark & 0.329 & \cmark & 0.325 \\
 & MiMo-VL-7B & \cmark & 0.448 & \cmark & 0.430 & \cmark & 0.431 & \cmark & 0.427 \\
 & TimeLens-8B & \cmark & 0.405 & \cmark & 0.391 & \cmark & 0.391 & \cmark & 0.389 \\
 & TimeLens2-4B & \cmark & 0.400 & \cmark & 0.381 & \cmark & 0.383 & \cmark & 0.381 \\
 & TimeLens2-8B & \cmark & 0.408 & \cmark & 0.390 & \cmark & 0.389 & \cmark & 0.385 \\
\midrule
QVHighlights & Qwen3-VL-4B & \cmark & 0.324 & \cmark & 0.255 & \cmark & 0.232 & \cmark & 0.227 \\
 & Qwen3-VL-8B & \cmark & 0.340 & \cmark & 0.272 & \cmark & 0.239 & \cmark & 0.229 \\
 & MiMo-VL-7B & \cmark & 0.529 & \cmark & 0.462 & \cmark & 0.432 & \cmark & 0.429 \\
 & TimeLens-8B & \cmark & 0.267 & \cmark & 0.222 & \cmark & 0.205 & \cmark & 0.198 \\
 & TimeLens2-4B & \cmark & 0.257 & \cmark & 0.210 & \cmark & 0.192 & \cmark & 0.187 \\
 & TimeLens2-8B & \cmark & 0.235 & \cmark & 0.194 & \cmark & 0.182 & \cmark & 0.181 \\
\midrule
ActivityNet Captions & Qwen3-VL-4B & \cmark & 0.551 & \cmark & 0.515 & \cmark & 0.499 & \cmark & 0.501 \\
 & Qwen3-VL-8B & \cmark & 0.509 & \cmark & 0.466 & \cmark & 0.447 & \cmark & 0.443 \\
 & MiMo-VL-7B & \cmark & 0.635 & \cmark & 0.599 & \cmark & 0.592 & \cmark & 0.591 \\
 & TimeLens-8B & \cmark & 0.551 & \cmark & 0.517 & \cmark & 0.503 & \cmark & 0.504 \\
 & TimeLens2-4B & \cmark & 0.544 & \cmark & 0.505 & \cmark & 0.488 & \cmark & 0.489 \\
 & TimeLens2-8B & \cmark & 0.521 & \cmark & 0.486 & \cmark & 0.468 & \cmark & 0.465 \\
\bottomrule
\end{tabular}
\end{adjustbox}


\end{table}
