# Supplementary material for: CAPTURE: Minimizing Watch Time for Reliable Temporal Video Grounding
Source: arXiv:2611.38466 source file (2026-11-28)
Supplement: Supplementary file 8 [file set_chlong.tex]

\begin{table*}[!t]
\caption{\textbf{On joined videos, \texttt{CAPTURE} watches less than calibrated single answers, but strict requests still require substantial viewing.}
TimeLens2-8B on 66 videos of about 10 minutes, over 1,000 trials with 18 calibration and 28 test videos.
Scoring is exact except in each block's last two rows, which use two prompts and their learned correction.
Hit and Watch follow \cref{sec:exp}.
Introduced methods meet each request on average.
With $n=18$, success is near $k_n/19$, for example 0.949 at 90\%.
A dash means whole-video fallback in more than 5\% of trials.
COVER~\cite{mohamed2026cover} calibrates whole-moment containment on queries.
\textbf{Bold} marks least watch duration among each block's first four rows.}
\label{tab:supp:chlong}
\hypertarget{table.caption.79}{}%
\centering
\scriptsize
\setlength{\tabcolsep}{2.2pt}
\begin{adjustbox}{max width=\textwidth}
\begin{tabular}{@{}l cc cc cc cc cc cc cc cc cc cc@{}}
\toprule
& \multicolumn{10}{c}{IoU\,$\ge$\,0.5 for} & \multicolumn{10}{c}{IoU\,$\ge$\,0.7 for} \\
\cmidrule(lr){2-11}\cmidrule(lr){12-21}
& \multicolumn{2}{c}{50\%} & \multicolumn{2}{c}{60\%} & \multicolumn{2}{c}{70\%} & \multicolumn{2}{c}{80\%} & \multicolumn{2}{c}{90\%} & \multicolumn{2}{c}{50\%} & \multicolumn{2}{c}{60\%} & \multicolumn{2}{c}{70\%} & \multicolumn{2}{c}{80\%} & \multicolumn{2}{c}{90\%} \\
\cmidrule(lr){2-3}\cmidrule(lr){4-5}\cmidrule(lr){6-7}\cmidrule(lr){8-9}\cmidrule(lr){10-11}\cmidrule(lr){12-13}\cmidrule(lr){14-15}\cmidrule(lr){16-17}\cmidrule(lr){18-19}\cmidrule(lr){20-21}
\textbf{Method} & Hit & Watch$\downarrow$ & Hit & Watch$\downarrow$ & Hit & Watch$\downarrow$ & Hit & Watch$\downarrow$ & Hit & Watch$\downarrow$ & Hit & Watch$\downarrow$ & Hit & Watch$\downarrow$ & Hit & Watch$\downarrow$ & Hit & Watch$\downarrow$ & Hit & Watch$\downarrow$ \\
\midrule
\multicolumn{21}{@{}l}{\textit{All 2,638 queries}} \\
Exact anchor with continuation & 0.529 & 0.088 & 0.636 & \best{0.163} & 0.741 & \best{0.273} & 0.844 & \best{0.449} & 0.949 & \best{0.741} & 0.527 & 0.106 & 0.635 & \best{0.181} & 0.740 & \best{0.291} & 0.842 & \best{0.464} & 0.950 & \best{0.758} \\
Per-second threshold & 0.530 & \best{0.081} & 0.644 & 0.164 & 0.755 & 0.301 & 0.859 & 0.488 & 0.956 & 0.764 & 0.532 & \best{0.095} & 0.645 & 0.184 & 0.757 & 0.328 & 0.860 & 0.515 & 0.956 & 0.780 \\
Calibrated greedy answer & 0.550 & 0.229 & 0.671 & 0.399 & 0.784 & 0.579 & -- & -- & -- & -- & 0.551 & 0.236 & 0.672 & 0.404 & 0.784 & 0.582 & -- & -- & -- & -- \\
MBR answer at $\tau$, calibrated scale & 0.548 & 0.215 & 0.668 & 0.388 & 0.781 & 0.574 & -- & -- & -- & -- & 0.550 & 0.222 & 0.669 & 0.391 & 0.783 & 0.575 & -- & -- & -- & -- \\
\gray{COVER~\cite{mohamed2026cover}} & \gray{0.514} & \gray{0.150} & \gray{0.607} & \gray{0.298} & \gray{0.707} & \gray{0.450} & \gray{0.806} & \gray{0.601} & \gray{0.904} & \gray{0.786} & \gray{0.509} & \gray{0.150} & \gray{0.604} & \gray{0.298} & \gray{0.705} & \gray{0.450} & \gray{0.804} & \gray{0.601} & \gray{0.903} & \gray{0.786} \\
Exact anchor, product from two prompts & 0.529 & 0.225 & 0.633 & 0.306 & 0.737 & 0.413 & 0.843 & 0.599 & 0.949 & 0.831 & 0.528 & 0.270 & 0.631 & 0.336 & 0.739 & 0.450 & 0.844 & 0.619 & 0.949 & 0.836 \\
Exact anchor, learned correction of this product & 0.531 & 0.094 & 0.636 & 0.168 & 0.740 & 0.291 & 0.841 & 0.453 & 0.948 & 0.754 & 0.529 & 0.118 & 0.635 & 0.184 & 0.742 & 0.298 & 0.840 & 0.464 & 0.947 & 0.770 \\
\midrule
\multicolumn{21}{@{}l}{\textit{The 1,796 queries whose verb and object recur in no other source video of the joined video}} \\
Exact anchor with continuation & 0.537 & 0.082 & 0.637 & \best{0.144} & 0.741 & \best{0.250} & 0.845 & \best{0.418} & 0.946 & \best{0.718} & 0.536 & 0.099 & 0.637 & \best{0.164} & 0.739 & \best{0.264} & 0.844 & \best{0.438} & 0.947 & \best{0.743} \\
Per-second threshold & 0.536 & \best{0.070} & 0.645 & \best{0.144} & 0.756 & 0.274 & 0.860 & 0.463 & 0.954 & 0.749 & 0.536 & \best{0.082} & 0.648 & \best{0.164} & 0.757 & 0.299 & 0.861 & 0.489 & 0.955 & 0.766 \\
Calibrated greedy answer & 0.551 & 0.194 & 0.666 & 0.362 & 0.779 & 0.555 & -- & -- & -- & -- & 0.552 & 0.203 & 0.666 & 0.368 & 0.780 & 0.558 & -- & -- & -- & -- \\
MBR answer at $\tau$, calibrated scale & 0.551 & 0.184 & 0.663 & 0.351 & 0.779 & 0.557 & 0.885 & 0.762 & -- & -- & 0.550 & 0.190 & 0.664 & 0.355 & 0.780 & 0.555 & -- & -- & -- & -- \\
\gray{COVER~\cite{mohamed2026cover}} & \gray{0.514} & \gray{0.117} & \gray{0.606} & \gray{0.246} & \gray{0.704} & \gray{0.420} & \gray{0.804} & \gray{0.586} & \gray{0.901} & \gray{0.784} & \gray{0.508} & \gray{0.117} & \gray{0.603} & \gray{0.246} & \gray{0.701} & \gray{0.420} & \gray{0.801} & \gray{0.586} & \gray{0.900} & \gray{0.784} \\
Exact anchor, product from two prompts & 0.532 & 0.220 & 0.635 & 0.302 & 0.739 & 0.404 & 0.845 & 0.593 & 0.948 & 0.823 & 0.529 & 0.247 & 0.634 & 0.327 & 0.743 & 0.447 & 0.846 & 0.616 & 0.948 & 0.826 \\
Exact anchor, learned correction of this product & 0.536 & 0.086 & 0.636 & 0.150 & 0.741 & 0.264 & 0.844 & 0.409 & 0.947 & 0.744 & 0.533 & 0.109 & 0.637 & 0.167 & 0.742 & 0.270 & 0.845 & 0.456 & 0.947 & 0.746 \\
\bottomrule
\end{tabular}
\end{adjustbox}


\end{table*}
