# Supplementary material for: CAPTURE: Minimizing Watch Time for Reliable Temporal Video Grounding
Source: arXiv:2611.38466 source file (2026-11-28)
Supplement: Supplementary file 9 [file set_fact.tex]

\begin{table*}[!t]
\caption{\textbf{Products of exact endpoint marginals give similar watch duration, while separate prompts benefit from a learned correction.}
Watch duration over 1,000 trials with the same exact-anchor construction, continuation rule and calibration procedure.
Joint rows repeat \cref{tab:supp:watch}.
Joint and product probabilities are normalized over scored spans.
The marginal product uses exact joint marginals, while two prompts score endpoints separately.
Correction training uses other benchmarks and target fit videos (\cref{sec:supp:impl:factorized}).
Top-peak rows retain spans overlapping any of the $k$ most probable peaks at tIoU $\ge0.5$, without renormalizing.
If retained probability is at most $q_0$, the construction budget increases to the video's full duration. The anchor uses retained spans inside the resulting region, and calibration determines how much is returned.
\textbf{Bold} marks least watch duration per model.}
\label{tab:supp:fact}
\centering
\scriptsize
\setlength{\tabcolsep}{3.2pt}
\begin{adjustbox}{max width=\textwidth}
\begin{tabular}{@{}ll cc cc cc@{}}
\toprule
& & \multicolumn{2}{c}{Charades-STA} & \multicolumn{2}{c}{QVHighlights} & \multicolumn{2}{c}{ActivityNet Captions} \\
\cmidrule(lr){3-4}\cmidrule(lr){5-6}\cmidrule(lr){7-8}
\textbf{Model} & \textbf{Span distribution} & 0.5, 80\% & 0.7, 80\% & 0.5, 80\% & 0.7, 80\% & 0.5, 80\% & 0.7, 80\% \\
\midrule
Qwen3-VL-4B & Joint, all spans & \best{0.34} & \best{0.43} & \best{0.24} & \best{0.32} & 0.48 & 0.57 \\
 & Product of the start and end marginals & 0.35 & 0.44 & \best{0.24} & 0.34 & \best{0.46} & 0.57 \\
 & Spans near the top peak & 0.42 & 0.47 & 0.33 & 0.41 & 0.48 & \best{0.48} \\
 & Spans near the top 2 peaks & 0.38 & 0.45 & 0.28 & 0.35 & 0.55 & 0.58 \\
 & Spans near the top 3 peaks & 0.38 & 0.45 & 0.27 & 0.34 & 0.53 & 0.61 \\
\midrule
TimeLens2-8B & Joint, all spans & 0.37 & 0.47 & \best{0.19} & \best{0.25} & 0.46 & \best{0.59} \\
 & Product of the start and end marginals & 0.37 & 0.47 & \best{0.19} & 0.26 & \best{0.45} & \best{0.59} \\
 & Product from two prompts & 0.40 & 0.53 & 0.22 & 0.31 & 0.49 & 0.62 \\
 & Learned correction of the two-prompt product & \best{0.35} & \best{0.45} & 0.20 & 0.26 & 0.46 & \best{0.59} \\
 & Spans near the top peak & 0.41 & 0.46 & 0.21 & 0.27 & 0.55 & 0.62 \\
 & Spans near the top 2 peaks & 0.43 & 0.49 & 0.20 & 0.26 & 0.53 & 0.62 \\
 & Spans near the top 3 peaks & 0.42 & 0.49 & 0.20 & 0.26 & 0.51 & 0.61 \\
\midrule
Qwen3-VL-8B & Joint, all spans & \best{0.31} & \best{0.42} & \best{0.23} & \best{0.31} & \best{0.44} & \best{0.54} \\
 & Product of the start and end marginals & 0.32 & \best{0.42} & \best{0.23} & \best{0.31} & \best{0.44} & 0.55 \\
\bottomrule
\end{tabular}
\end{adjustbox}


\end{table*}
