# Supplementary material for: CAPTURE: Minimizing Watch Time for Reliable Temporal Video Grounding
Source: arXiv:2611.38466 source file (2026-11-28)
Supplement: Supplementary file 10 [file set_methods_full.tex]

\begin{table*}[!t]
\caption{\textbf{Extended QVHighlights comparison: a \texttt{CAPTURE} region type watches least in all six settings among methods with the same guarantee.}
Results use 1,000 trials.
Greedy has no guarantee (\xmark), and Hit treats its answer as one region.
COVER~\cite{mohamed2026cover}, the prior method, calibrates whole-moment containment on queries.
Baselines and \texttt{CAPTURE} region types share our video-level guarantee.
Exact anchor (main paper) uses the configuration of \cref{tab:main,tab:methods} but comes from a separate run; \cref{tab:main,tab:methods} differ from it by at most 0.01 in Hit and Watch and 0.12 in Seg.
Anchor-based variants select $q_0$ on all fit videos.
Cal. reports how often fallback is avoided (\cmark\ means all trials), counting both outputs of \emph{Greedy answer or whole video}.
Cal. is not reported for the prior method (--).
Hit, Watch and Seg. follow \cref{sec:exp}, averaged over trials without fallback.
\textbf{Bold} marks least watch duration among guaranteed methods with fallback in at most 5\% of trials.}
\label{tab:supp:methods}
\hypertarget{table.caption.70}{}%
\centering
\scriptsize
\setlength{\tabcolsep}{2.2pt}
\begin{adjustbox}{max width=\textwidth}
\begin{tabular}{@{}l cccccc cccccc cccccc@{}}
\toprule
& \multicolumn{6}{c}{\textbf{Qwen3-VL-4B}} & \multicolumn{6}{c}{\textbf{TimeLens2-8B}} & \multicolumn{6}{c}{\textbf{Qwen3-VL-8B}} \\
\cmidrule(lr){2-7}\cmidrule(lr){8-13}\cmidrule(lr){14-19}
& \multicolumn{4}{c}{0.5, 80\%} & \multicolumn{2}{c}{0.7, 80\%} & \multicolumn{4}{c}{0.5, 80\%} & \multicolumn{2}{c}{0.7, 80\%} & \multicolumn{4}{c}{0.5, 80\%} & \multicolumn{2}{c}{0.7, 80\%} \\
\cmidrule(lr){2-5}\cmidrule(lr){6-7}\cmidrule(lr){8-11}\cmidrule(lr){12-13}\cmidrule(lr){14-17}\cmidrule(lr){18-19}
\textbf{Method} & Cal. & Hit & Watch$\downarrow$ & Seg. & Cal. & Watch$\downarrow$ & Cal. & Hit & Watch$\downarrow$ & Seg. & Cal. & Watch$\downarrow$ & Cal. & Hit & Watch$\downarrow$ & Seg. & Cal. & Watch$\downarrow$ \\
\midrule
\multicolumn{19}{@{}l}{\textit{Prior methods}} \\
\gray{Greedy answer of the model} & \xmark & \gray{0.75} & \gray{0.27} & \gray{1.00} & \xmark & \gray{0.27} & \xmark & \gray{0.88} & \gray{0.29} & \gray{1.00} & \xmark & \gray{0.29} & \xmark & \gray{0.74} & \gray{0.25} & \gray{1.00} & \xmark & \gray{0.25} \\
\gray{COVER~\cite{mohamed2026cover}} & -- & \gray{0.93} & \gray{0.71} & \gray{1.00} & -- & \gray{0.71} & -- & \gray{0.96} & \gray{0.55} & \gray{1.00} & -- & \gray{0.55} & -- & \gray{0.92} & \gray{0.71} & \gray{1.00} & -- & \gray{0.71} \\
\midrule
\multicolumn{19}{@{}l}{\textit{Baselines}} \\
Positional prior, no model & \cmark & 0.83 & 0.77 & 2.78 & \cmark & 0.87 & \cmark & 0.83 & 0.77 & 2.78 & \cmark & 0.87 & \cmark & 0.83 & 0.77 & 2.78 & \cmark & 0.87 \\
Greedy answer or whole video & \cmark & 0.99 & 0.96 & 1.00 & \cmark & 1.00 & \cmark & 0.88 & 0.30 & 1.00 & \cmark & 0.50 & \cmark & 0.99 & 0.97 & 1.00 & \cmark & 1.00 \\
Calibrated greedy answer & \cmark & 0.81 & 0.37 & 1.00 & \cmark & 0.46 & \cmark & 0.83 & 0.22 & 1.00 & \cmark & 0.29 & \cmark & 0.81 & 0.37 & 1.00 & \cmark & 0.46 \\
MBR answer at $\tau$, calibrated scale & \cmark & 0.81 & 0.30 & 1.00 & \cmark & 0.42 & \cmark & 0.83 & 0.21 & 1.00 & \cmark & 0.28 & \cmark & 0.82 & 0.23 & 1.00 & \cmark & 0.34 \\
\midrule
\multicolumn{19}{@{}l}{\textit{\texttt{CAPTURE} region types}} \\
Per-second threshold & \cmark & 0.81 & 0.30 & 1.05 & \cmark & 0.34 & \cmark & 0.81 & 0.24 & 0.97 & \cmark & 0.28 & \cmark & 0.81 & 0.27 & 1.04 & \cmark & 0.30 \\
Enumerate-and-cover order & \cmark & 0.80 & \best{0.23} & 1.10 & \cmark & \best{0.31} & \cmark & 0.91 & 0.25 & 1.00 & \cmark & 0.27 & \cmark & 0.82 & \best{0.22} & 1.04 & \cmark & \best{0.29} \\
Gain-per-second anchor & \cmark & 0.80 & 0.24 & 1.35 & \cmark & 0.32 & \cmark & 0.81 & \best{0.18} & 1.02 & \cmark & 0.27 & \cmark & 0.81 & 0.25 & 1.35 & \cmark & 0.30 \\
Exact anchor (main paper) & \cmark & 0.81 & 0.24 & 1.28 & \cmark & 0.32 & \cmark & 0.81 & 0.19 & 1.03 & \cmark & \best{0.25} & \cmark & 0.80 & 0.23 & 1.27 & \cmark & 0.31 \\
Exact anchor with continuation & \cmark & 0.81 & 0.24 & 1.28 & \cmark & 0.32 & \cmark & 0.81 & 0.19 & 1.03 & \cmark & \best{0.25} & \cmark & 0.80 & 0.23 & 1.27 & \cmark & 0.31 \\
\bottomrule
\end{tabular}
\end{adjustbox}


\end{table*}
