# Supplementary material for: CAPTURE: Minimizing Watch Time for Reliable Temporal Video Grounding
Source: arXiv:2611.38466 source file (2026-11-28)
Supplement: Supplementary file 11 [file set_newpools.tex]

\begin{table*}[!t]
\caption{\textbf{On two benchmarks with code and settings fixed before evaluation, \texttt{CAPTURE} watches less than the prior method~\cite{mohamed2026cover} and the calibrated greedy answer at all six requests.}
Watch duration over 1,000 trials on Charades-TimeLens and ActivityNet-TimeLens~\cite{zhang2025timelens}.
Results use the region type selected on fit videos, an ablation rather than the main-paper configuration; across the cells of \cref{tab:main}, the two differ by 0.018 in mean normalized watch duration and by at most 0.075.
\textbf{Bold} marks the shortest watch duration among methods with \texttt{CAPTURE}'s guarantee.}
\label{tab:supp:newpools}
\hypertarget{table.caption.81}{}%
\centering
\scriptsize
\setlength{\tabcolsep}{3.2pt}
\begin{adjustbox}{max width=\textwidth}
\begin{tabular}{@{}lll cccccc@{}}
\toprule
& & & \multicolumn{3}{c}{IoU\,$\ge$\,0.5 for} & \multicolumn{3}{c}{IoU\,$\ge$\,0.7 for} \\
\cmidrule(lr){4-6}\cmidrule(lr){7-9}
\textbf{Benchmark} & \textbf{Model} & \textbf{Method} & 70\% & 80\% & 90\% & 70\% & 80\% & 90\% \\
\midrule
Charades-TimeLens & TimeLens2-8B & Region type selected on fit videos & \best{0.15} & \best{0.18} & \best{0.26} & \best{0.23} & \best{0.28} & \best{0.36} \\
 &  & Calibrated greedy answer & 0.20 & 0.25 & 0.35 & 0.26 & 0.31 & 0.42 \\
 &  & Per-second threshold & 0.19 & 0.23 & 0.30 & 0.25 & 0.29 & 0.37 \\
 &  & Positional prior & 0.67 & 0.76 & 0.86 & 0.77 & 0.84 & 0.90 \\
 &  & \gray{COVER~\cite{mohamed2026cover}} & \gray{0.33} & \gray{0.37} & \gray{0.50} & \gray{0.33} & \gray{0.37} & \gray{0.50} \\
\cmidrule(lr){2-9}
 & Qwen3-VL-8B & Region type selected on fit videos & \best{0.18} & \best{0.23} & \best{0.34} & \best{0.26} & \best{0.32} & \best{0.41} \\
 &  & Calibrated greedy answer & 0.21 & 0.28 & 0.54 & 0.27 & 0.33 & 0.63 \\
 &  & Per-second threshold & 0.20 & 0.26 & 0.37 & \best{0.26} & \best{0.32} & 0.43 \\
 &  & Positional prior & 0.67 & 0.76 & 0.86 & 0.77 & 0.84 & 0.90 \\
 &  & \gray{COVER~\cite{mohamed2026cover}} & \gray{0.32} & \gray{0.38} & \gray{0.63} & \gray{0.32} & \gray{0.38} & \gray{0.63} \\
\midrule
ActivityNet-TimeLens & TimeLens2-8B & Region type selected on fit videos & \best{0.12} & \best{0.17} & \best{0.25} & \best{0.17} & \best{0.22} & \best{0.31} \\
 &  & Calibrated greedy answer & 0.17 & 0.27 & 0.60 & 0.21 & 0.31 & 0.62 \\
 &  & Per-second threshold & 0.16 & 0.21 & 0.33 & 0.20 & 0.24 & 0.35 \\
 &  & Positional prior & 0.84 & 0.91 & 0.94 & 0.91 & 0.92 & 0.96 \\
 &  & \gray{COVER~\cite{mohamed2026cover}} & \gray{0.22} & \gray{0.31} & \gray{0.59} & \gray{0.22} & \gray{0.31} & \gray{0.59} \\
\bottomrule
\end{tabular}
\end{adjustbox}


\end{table*}
