# Supplementary material for: CAPTURE: Minimizing Watch Time for Reliable Temporal Video Grounding
Source: arXiv:2611.38466 source file (2026-11-28)
Supplement: Supplementary file 12 [file set_quality.tex]

\begin{table*}[!t]
\caption{\textbf{\texttt{CAPTURE} returns more precise footage, while widened answers contain whole moments more often.}
Means across six models at tIoU 0.5 and 80\% requested success, over 1,000 trials.
Overlap measures use the region's best-matching annotated moment.
Precision divides overlap by watch duration, Recall by moment duration, and IoU by their union.
Contained measures how often a whole moment is included.
Annotations are clipped to video boundaries (\cref{sec:supp:impl:baselines}).
Greedy Hit treats the answer as one region.
A missing answer gives it an empty region and zero overlap scores, while the prior method and calibrated greedy answer return the full video.
Only introduced methods have our video-level matching-clip guarantee.
On Charades-STA, fit-video selection picks per-second thresholding for all six models.
Results use the region type selected on fit videos, an ablation rather than the main-paper configuration; across the cells of \cref{tab:main}, the two differ by 0.018 in mean normalized watch duration and by at most 0.075.}
\label{tab:supp:quality}
\hypertarget{table.caption.73}{}%
\centering
\scriptsize
\setlength{\tabcolsep}{2.6pt}
\begin{adjustbox}{max width=\textwidth}
\begin{tabular}{@{}llcccccc@{}}
\toprule
\textbf{Benchmark} & \textbf{Method} & Hit & Watch$\downarrow$ & IoU$\uparrow$ & Precision$\uparrow$ & Recall$\uparrow$ & Contained \\
\midrule
Charades-STA & \gray{Greedy answer of the model} & \gray{0.60} & \gray{0.25} & \gray{0.46} & \gray{0.70} & \gray{0.55} & \gray{0.11} \\
 & \gray{COVER~\cite{mohamed2026cover}} & \gray{0.91} & \gray{0.58} & \gray{0.45} & \gray{0.47} & \gray{0.90} & \gray{0.80} \\
 & Calibrated greedy answer & 0.81 & 0.38 & 0.54 & 0.64 & 0.76 & 0.41 \\
 & Per-second threshold & 0.80 & 0.33 & 0.53 & 0.68 & 0.70 & 0.19 \\
 & Exact anchor with continuation & 0.81 & 0.38 & 0.48 & 0.63 & 0.71 & 0.22 \\
 & Region type selected on fit videos & 0.80 & 0.33 & 0.53 & 0.68 & 0.70 & 0.19 \\
\midrule
QVHighlights & \gray{Greedy answer of the model} & \gray{0.78} & \gray{0.25} & \gray{0.60} & \gray{0.74} & \gray{0.73} & \gray{0.27} \\
 & \gray{COVER~\cite{mohamed2026cover}} & \gray{0.94} & \gray{0.65} & \gray{0.34} & \gray{0.35} & \gray{0.94} & \gray{0.90} \\
 & Calibrated greedy answer & 0.82 & 0.31 & 0.52 & 0.66 & 0.76 & 0.45 \\
 & Per-second threshold & 0.81 & 0.28 & 0.59 & 0.72 & 0.75 & 0.31 \\
 & Exact anchor with continuation & 0.81 & 0.25 & 0.49 & 0.71 & 0.66 & 0.22 \\
 & Region type selected on fit videos & 0.81 & 0.24 & 0.48 & 0.71 & 0.65 & 0.23 \\
\midrule
ActivityNet Captions & \gray{Greedy answer of the model} & \gray{0.57} & \gray{0.33} & \gray{0.42} & \gray{0.63} & \gray{0.57} & \gray{0.21} \\
 & \gray{COVER~\cite{mohamed2026cover}} & \gray{0.88} & \gray{0.69} & \gray{0.40} & \gray{0.43} & \gray{0.88} & \gray{0.80} \\
 & Calibrated greedy answer & 0.82 & 0.60 & 0.42 & 0.49 & 0.81 & 0.69 \\
 & Per-second threshold & 0.80 & 0.52 & 0.48 & 0.57 & 0.77 & 0.37 \\
 & Exact anchor with continuation & 0.82 & 0.50 & 0.42 & 0.55 & 0.75 & 0.28 \\
 & Region type selected on fit videos & 0.80 & 0.48 & 0.44 & 0.56 & 0.74 & 0.30 \\
\bottomrule
\end{tabular}
\end{adjustbox}


\end{table*}
