# Supplementary material for: CAPTURE: Minimizing Watch Time for Reliable Temporal Video Grounding
Source: arXiv:2611.38466 source file (2026-11-28)
Supplement: Supplementary file 13 [file set_retarget.tex]

\begin{table*}[!t]
\caption{\textbf{Calibrating COVER for one matching clip removes most of the original gap. \texttt{CAPTURE} still watches less in 86 of 108 cells.}
Mean watch duration over 18 model--benchmark pairs and 1,000 trials.
Retargeted COVER modifies the prior method~\cite{mohamed2026cover} as described in \cref{sec:supp:results:fair}.
Calibrating on videos gives our marginal guarantee but not the exact-anchor watch-duration bound.
The queries-as-units row uses all calibration queries.
The prior method keeps query-level calibration and whole-moment containment.
Retargeted mean success is at most 0.001 below each request.
\textbf{Bold} marks least watch duration among methods with our video-level guarantee.}
\label{tab:supp:retarget}
\centering
\scriptsize
\setlength{\tabcolsep}{3pt}
\begin{tabular}{@{}l cccccc@{}}
\toprule
& \multicolumn{3}{c}{IoU\,$\ge$\,0.5 for} & \multicolumn{3}{c}{IoU\,$\ge$\,0.7 for} \\
\cmidrule(lr){2-4}\cmidrule(lr){5-7}
\textbf{Method} & 70\% & 80\% & 90\% & 70\% & 80\% & 90\% \\
\midrule
\gray{COVER~\cite{mohamed2026cover}, whole moment} & \gray{0.536} & \gray{0.646} & \gray{0.800} & \gray{0.536} & \gray{0.646} & \gray{0.800} \\
\midrule
COVER, retargeted to IoU $\tau$ & 0.325 & 0.416 & 0.596 & 0.397 & 0.493 & 0.666 \\
COVER, retargeted, queries as units & 0.323 & 0.409 & 0.588 & 0.394 & 0.485 & 0.659 \\
\midrule
Calibrated greedy answer & 0.335 & 0.430 & 0.626 & 0.411 & 0.518 & 0.702 \\
\texttt{CAPTURE}, exact anchor & \best{0.291} & \best{0.371} & \best{0.498} & \best{0.384} & \best{0.462} & \best{0.581} \\
\midrule
\textit{Pairs where \texttt{CAPTURE} watches less than retargeted COVER} & 15 & 14 & 16 & 12 & 14 & 15 \\
\bottomrule
\end{tabular}
\end{table*}
