# Supplementary material for: CAPTURE: Minimizing Watch Time for Reliable Temporal Video Grounding
Source: arXiv:2611.38466 source file (2026-11-28)
Supplement: Supplementary file 14 [file set_runtime.tex]

\begin{table*}[!t]
\caption{\textbf{Scoring all spans takes 0.7 to 5.6 times as long as greedy decoding.}
Median seconds for 20 test queries per model and benchmark on an idle H200 GPU.
Video decoding is shared and excluded from subsequent rows.
The prior method and calibrated greedy answer each generate one answer.
Full-distribution MBR and span-based region types score every span.
Region construction adds a median 0.08 seconds.
The positional prior uses no model, and one-time calibration is excluded.}
\label{tab:supp:runtime}
\centering
\scriptsize
\setlength{\tabcolsep}{2.4pt}
\begin{tabular}{@{}l cc cc cc@{}}
\toprule
& \multicolumn{2}{c}{Charades-STA} & \multicolumn{2}{c}{QVHighlights} & \multicolumn{2}{c}{ActivityNet Captions} \\
\cmidrule(lr){2-3}\cmidrule(lr){4-5}\cmidrule(lr){6-7}
\textbf{Seconds per query} & Qwen3-VL-4B & TimeLens2-8B & Qwen3-VL-4B & TimeLens2-8B & Qwen3-VL-4B & TimeLens2-8B \\
\midrule
\gray{Video decoding, shared by methods that run the model} & \gray{0.71} & \gray{0.75} & \gray{3.75} & \gray{3.82} & \gray{5.57} & \gray{5.77} \\
\midrule
Greedy answer, COVER and calibrated greedy answer & 0.70 & 0.72 & 1.32 & 1.56 & 1.25 & 1.49 \\
\texttt{CAPTURE}, all spans & 0.48 & 0.56 & 7.35 & 7.96 & 3.17 & 3.43 \\
\bottomrule
\end{tabular}


\end{table*}
