# Supplementary material for: CAPTURE: Minimizing Watch Time for Reliable Temporal Video Grounding
Source: arXiv:2611.38466 source file (2026-11-28)
Supplement: Supplementary file 15 [file set_size.tex]

\begin{table*}[!t]
\caption{\textbf{\texttt{CAPTURE} watches less than the prior method~\cite{mohamed2026cover} and the calibrated greedy answer across seven Qwen3-VL and TimeLens2 models, from 2B to 32B parameters.}
Watch duration at two of six requests over 1,000 trials, using the region type selected on fit videos, an ablation that differs from the main-paper configuration by 0.018 on average and at most 0.075 across the cells of \cref{tab:main}.
All methods average over each trial's test queries and then over trials, whereas \cref{tab:main} averages over test videos; the calibrated greedy answer comes from a different run than the greedy anchor of \cref{tab:methods}.
\textbf{Bold} marks the shortest watch duration within each model family.}
\label{tab:supp:size}
\hypertarget{table.caption.82}{}%
\centering
\scriptsize
\setlength{\tabcolsep}{2.0pt}
\begin{adjustbox}{max width=\textwidth}
\begin{tabular}{@{}l *{18}{c}@{}}
\toprule
 & \multicolumn{6}{c}{COVER~\cite{mohamed2026cover}} & \multicolumn{6}{c}{Calibrated greedy answer} & \multicolumn{6}{c}{Region type selected on fit videos} \\
\cmidrule(lr){2-7}\cmidrule(lr){8-13}\cmidrule(lr){14-19}
 & \multicolumn{2}{c}{Charades-STA} & \multicolumn{2}{c}{QVHighlights} & \multicolumn{2}{c}{ActivityNet Captions} & \multicolumn{2}{c}{Charades-STA} & \multicolumn{2}{c}{QVHighlights} & \multicolumn{2}{c}{ActivityNet Captions} & \multicolumn{2}{c}{Charades-STA} & \multicolumn{2}{c}{QVHighlights} & \multicolumn{2}{c}{ActivityNet Captions} \\
\cmidrule(lr){2-3}\cmidrule(lr){4-5}\cmidrule(lr){6-7}\cmidrule(lr){8-9}\cmidrule(lr){10-11}\cmidrule(lr){12-13}\cmidrule(lr){14-15}\cmidrule(lr){16-17}\cmidrule(lr){18-19}
\textbf{Model} & 0.5, 80\% & 0.7, 80\% & 0.5, 80\% & 0.7, 80\% & 0.5, 80\% & 0.7, 80\% & 0.5, 80\% & 0.7, 80\% & 0.5, 80\% & 0.7, 80\% & 0.5, 80\% & 0.7, 80\% & 0.5, 80\% & 0.7, 80\% & 0.5, 80\% & 0.7, 80\% & 0.5, 80\% & 0.7, 80\% \\
\midrule
Qwen3-VL-2B & \gray{0.62} & \gray{0.62} & \gray{0.76} & \gray{0.76} & \gray{0.74} & \gray{0.74} & 0.46 & 0.57 & 0.38 & 0.48 & 0.65 & 0.72 & 0.35 & 0.46 & 0.24 & 0.32 & 0.52 & 0.62 \\
Qwen3-VL-4B & \gray{0.58} & \gray{0.58} & \gray{0.72} & \gray{0.72} & \gray{0.68} & \gray{0.68} & 0.38 & 0.50 & 0.37 & 0.46 & 0.58 & 0.66 & 0.31 & 0.40 & 0.24 & 0.32 & 0.47 & 0.56 \\
Qwen3-VL-8B & \gray{0.54} & \gray{0.54} & \gray{0.72} & \gray{0.72} & \gray{0.68} & \gray{0.68} & 0.34 & 0.46 & 0.37 & 0.46 & 0.57 & 0.65 & 0.31 & 0.40 & 0.22 & 0.30 & 0.44 & 0.55 \\
Qwen3-VL-32B & \gray{0.52} & \gray{0.52} & \gray{0.73} & \gray{0.73} & \gray{0.65} & \gray{0.65} & 0.31 & 0.41 & 0.34 & 0.43 & 0.54 & 0.62 & \best{0.29} & \best{0.38} & \best{0.21} & \best{0.29} & \best{0.40} & \best{0.50} \\
\midrule
TimeLens2-2B & \gray{0.61} & \gray{0.61} & \gray{0.60} & \gray{0.60} & \gray{0.68} & \gray{0.68} & 0.41 & 0.51 & 0.25 & 0.32 & 0.60 & 0.66 & 0.38 & 0.48 & 0.19 & 0.27 & 0.48 & 0.60 \\
TimeLens2-4B & \gray{0.58} & \gray{0.58} & \gray{0.58} & \gray{0.58} & \gray{0.67} & \gray{0.67} & 0.37 & 0.49 & 0.22 & 0.29 & 0.59 & 0.65 & \best{0.34} & \best{0.45} & 0.19 & 0.26 & \best{0.46} & \best{0.58} \\
TimeLens2-8B & \gray{0.58} & \gray{0.58} & \gray{0.55} & \gray{0.55} & \gray{0.67} & \gray{0.67} & 0.37 & 0.48 & 0.22 & 0.29 & 0.58 & 0.64 & 0.35 & 0.47 & \best{0.18} & \best{0.25} & \best{0.46} & 0.59 \\
\bottomrule
\end{tabular}
\end{adjustbox}
\end{table*}
