# Supplementary material for: CAPTURE: Minimizing Watch Time for Reliable Temporal Video Grounding
Source: arXiv:2611.38466 source file (2026-11-28)
Supplement: Supplementary file 16 [file set_tau1.tex]

\begin{table*}[!t]
\caption{\textbf{For whole-moment containment, \texttt{CAPTURE} watches more than the prior method at 70\% but less from 80\%.}
Means over 18 model--benchmark pairs and 1,000 trials.
At $\tau=1$, all methods clip annotations at $\lfloor T\rfloor$.
Calibrated rows show watch duration with empirical success in parentheses.
Introduced methods calibrate on videos, the prior method~\cite{mohamed2026cover} on queries.
Comparisons at matched empirical success use test annotations to choose thresholds within each query group, so cannot be deployed.
\Cref{sec:supp:results:fair} defines wrong-peak queries.
\textbf{Bold} marks least watch duration per column and block.}
\label{tab:supp:tau1}
\centering
\scriptsize
\setlength{\tabcolsep}{3pt}
\begin{tabular}{@{}ll ccccc@{}}
\toprule
\textbf{Queries} & \textbf{Method} & 70\% & 80\% & 85\% & 90\% & 95\% \\
\midrule
\multicolumn{7}{@{}l}{\textit{$\tau=1$, calibrated at the requested rate, all test videos, watch (hit)}} \\
All & COVER~\cite{mohamed2026cover} & 0.53 (0.74) & 0.65 (0.83) & 0.72 (0.87) & 0.80 (0.92) & 0.90 (0.96) \\
 & Calibrated greedy answer & \best{0.51} (0.73) & \best{0.62} (0.83) & 0.69 (0.87) & 0.78 (0.92) & 0.90 (0.96) \\
 & \texttt{CAPTURE}, exact anchor & 0.56 (0.70) & 0.63 (0.80) & 0.67 (0.85) & \best{0.72} (0.90) & \best{0.80} (0.95) \\
 & \texttt{CAPTURE}, gain-per-second order & 0.56 (0.70) & 0.63 (0.80) & \best{0.66} (0.85) & \best{0.72} (0.90) & \best{0.80} (0.95) \\
 & \textit{Pairs where \texttt{CAPTURE} watches less than the prior method} & 4 & 8 & 9 & 11 & 13 \\
\midrule
\multicolumn{7}{@{}l}{\textit{$\tau=1$, matched empirical success within groups, watch}} \\
Wrong peak & COVER~\cite{mohamed2026cover} & 0.60 & 0.67 & 0.72 & 0.78 & 0.87 \\
 & Calibrated greedy answer & 0.63 & 0.71 & 0.76 & 0.81 & 0.90 \\
 & \texttt{CAPTURE}, exact anchor & 0.60 & 0.66 & 0.69 & 0.74 & 0.81 \\
 & \texttt{CAPTURE}, gain-per-second order & \best{0.59} & \best{0.65} & \best{0.68} & \best{0.73} & \best{0.80} \\
 & \textit{Pairs where \texttt{CAPTURE} watches less than the prior method} & 5 & 11 & 12 & 16 & 16 \\
\cmidrule(lr){2-7}
Other & COVER~\cite{mohamed2026cover} & \best{0.48} & \best{0.56} & \best{0.62} & 0.72 & 0.84 \\
 & Calibrated greedy answer & 0.49 & 0.59 & 0.65 & 0.74 & 0.87 \\
 & \texttt{CAPTURE}, exact anchor & 0.56 & 0.62 & 0.66 & 0.72 & 0.79 \\
 & \texttt{CAPTURE}, gain-per-second order & 0.55 & 0.62 & 0.66 & \best{0.71} & \best{0.78} \\
 & \textit{Pairs where \texttt{CAPTURE} watches less than the prior method} & 0 & 3 & 4 & 8 & 11 \\
\midrule
\multicolumn{7}{@{}l}{\textit{$\tau=0.5$, for comparison}} \\
All, calibrated & COVER~\cite{mohamed2026cover} & 0.54 (0.87) & 0.65 (0.91) & 0.72 (0.93) & 0.80 (0.95) & 0.90 (0.98) \\
 & Calibrated greedy answer & 0.34 (0.72) & 0.43 (0.82) & 0.51 (0.86) & 0.63 (0.91) & 0.81 (0.96) \\
 & \texttt{CAPTURE}, exact anchor & \best{0.29} (0.70) & \best{0.37} (0.80) & \best{0.42} (0.85) & \best{0.50} (0.90) & \best{0.61} (0.95) \\
 & \textit{Pairs where \texttt{CAPTURE} watches less than the prior method} & 18 & 18 & 18 & 18 & 18 \\
\cmidrule(lr){2-7}
Wrong peak & COVER~\cite{mohamed2026cover} & 0.41 & 0.49 & 0.55 & 0.63 & 0.78 \\
 & Calibrated greedy answer & 0.42 & 0.52 & 0.58 & 0.66 & 0.81 \\
 & \texttt{CAPTURE}, exact anchor & \best{0.33} & \best{0.37} & \best{0.40} & \best{0.44} & \best{0.52} \\
 & \textit{Pairs where \texttt{CAPTURE} watches less than the prior method} & 17 & 17 & 18 & 18 & 18 \\
\cmidrule(lr){2-7}
Other & COVER~\cite{mohamed2026cover} & 0.34 & 0.40 & 0.46 & 0.57 & 0.75 \\
 & Calibrated greedy answer & 0.32 & 0.40 & 0.47 & 0.59 & 0.79 \\
 & \texttt{CAPTURE}, exact anchor & \best{0.30} & \best{0.37} & \best{0.43} & \best{0.51} & \best{0.61} \\
 & \textit{Pairs where \texttt{CAPTURE} watches less than the prior method} & 15 & 12 & 12 & 14 & 18 \\
\bottomrule
\end{tabular}
\end{table*}
