# Supplementary material for: CAPTURE: Minimizing Watch Time for Reliable Temporal Video Grounding
Source: arXiv:2611.38466 source file (2026-11-28)
Supplement: Supplementary file 17 [file set_units.tex]

\begin{table*}[!t]
\caption{\textbf{Calibrating on queries instead of videos gives mean empirical success more than 0.002 below the request in 22 of 72 cells.}
Entries give mean video-weighted test success minus the requested rate over 1,000 trials.
Video-level calibration draws one random query per video (\cref{alg:capture_calibration}).
Query-level calibration treats all queries as exchangeable, ignoring dependence within a video.
With videos as units, every entry is at least $-0.001$.
\textbf{Bold} marks entries below $-0.002$.
Results use the region type selected on fit videos, an ablation rather than the main-paper configuration; across the cells of \cref{tab:main}, the two differ by 0.018 in mean normalized watch duration and by at most 0.075.}
\label{tab:supp:units}
\centering
\scriptsize
\setlength{\tabcolsep}{2.0pt}
\begin{adjustbox}{max width=\textwidth}
\begin{tabular}{@{}ll cc cc cc cc@{}}
\toprule
& & \multicolumn{2}{c}{0.5, 70\%} & \multicolumn{2}{c}{0.5, 80\%} & \multicolumn{2}{c}{0.7, 70\%} & \multicolumn{2}{c}{0.7, 80\%} \\
\cmidrule(lr){3-4}\cmidrule(lr){5-6}\cmidrule(lr){7-8}\cmidrule(lr){9-10}
\textbf{Benchmark} & \textbf{Model} & Videos & Queries & Videos & Queries & Videos & Queries & Videos & Queries \\
\midrule
Charades-STA & Qwen3-VL-4B & $0.008$ & $0.002$ & $-0.001$ & $\mathbf{-0.008}$ & $0.001$ & $\mathbf{-0.003}$ & $0.000$ & $\mathbf{-0.003}$ \\
 & Qwen3-VL-8B & $0.000$ & $\mathbf{-0.013}$ & $-0.001$ & $\mathbf{-0.011}$ & $0.002$ & $-0.001$ & $0.001$ & $-0.001$ \\
 & MiMo-VL-7B & $0.002$ & $0.006$ & $0.001$ & $0.008$ & $0.004$ & $0.014$ & $0.003$ & $0.006$ \\
 & TimeLens-8B & $0.001$ & $0.001$ & $0.000$ & $-0.001$ & $0.001$ & $0.003$ & $0.003$ & $0.009$ \\
 & TimeLens2-4B & $0.005$ & $0.003$ & $0.001$ & $0.011$ & $0.000$ & $0.005$ & $0.002$ & $0.010$ \\
 & TimeLens2-8B & $0.009$ & $0.006$ & $0.000$ & $0.011$ & $0.000$ & $0.007$ & $-0.001$ & $-0.001$ \\
\midrule
QVHighlights & Qwen3-VL-4B & $0.001$ & $\mathbf{-0.002}$ & $0.006$ & $0.003$ & $0.001$ & $-0.001$ & $0.007$ & $0.005$ \\
 & Qwen3-VL-8B & $0.001$ & $-0.001$ & $0.017$ & $0.009$ & $0.002$ & $\mathbf{-0.004}$ & $0.006$ & $\mathbf{-0.002}$ \\
 & MiMo-VL-7B & $0.000$ & $0.009$ & $0.004$ & $0.004$ & $0.004$ & $0.011$ & $0.004$ & $0.005$ \\
 & TimeLens-8B & $0.000$ & $\mathbf{-0.010}$ & $0.005$ & $\mathbf{-0.004}$ & $0.015$ & $0.008$ & $0.005$ & $\mathbf{-0.002}$ \\
 & TimeLens2-4B & $-0.001$ & $0.011$ & $0.004$ & $-0.001$ & $0.000$ & $0.001$ & $0.005$ & $\mathbf{-0.003}$ \\
 & TimeLens2-8B & $0.049$ & $0.047$ & $0.008$ & $0.002$ & $0.006$ & $0.001$ & $0.006$ & $0.006$ \\
\midrule
ActivityNet Captions & Qwen3-VL-4B & $0.002$ & $\mathbf{-0.002}$ & $0.004$ & $\mathbf{-0.004}$ & $0.001$ & $\mathbf{-0.003}$ & $0.003$ & $\mathbf{-0.003}$ \\
 & Qwen3-VL-8B & $0.000$ & $\mathbf{-0.003}$ & $0.005$ & $-0.001$ & $0.000$ & $-0.002$ & $0.004$ & $\mathbf{-0.002}$ \\
 & MiMo-VL-7B & $0.003$ & $0.012$ & $0.005$ & $0.001$ & $0.001$ & $-0.001$ & $0.004$ & $\mathbf{-0.003}$ \\
 & TimeLens-8B & $0.002$ & $-0.002$ & $0.004$ & $\mathbf{-0.003}$ & $0.002$ & $-0.002$ & $0.004$ & $-0.001$ \\
 & TimeLens2-4B & $0.002$ & $-0.002$ & $0.004$ & $-0.001$ & $0.002$ & $0.000$ & $0.004$ & $0.000$ \\
 & TimeLens2-8B & $0.002$ & $0.000$ & $0.004$ & $\mathbf{-0.003}$ & $0.002$ & $-0.002$ & $0.004$ & $\mathbf{-0.004}$ \\
\bottomrule
\end{tabular}
\end{adjustbox}


\end{table*}
