# Supplementary material for: CAPTURE: Minimizing Watch Time for Reliable Temporal Video Grounding
Source: arXiv:2611.38466 source file (2026-11-28)
Supplement: Supplementary file 18 [file set_watch.tex]

\begin{table*}[!t]
\caption{\textbf{Region constructions compared with the same span probabilities and success guarantee.}
Results use video-level split-conformal calibration over 1,000 trials.
\Cref{tab:supp:methods} defines the metrics.
Span-ordering types share the model-estimated success stopping rule, while per-second thresholding constructs regions directly (\cref{sec:supp:watch}).
Exact anchor (main paper) uses the configuration of \cref{tab:main,tab:methods} but comes from a separate run; \cref{tab:main} differs from it by at most 0.01 in Hit, 0.02 in Watch and 0.12 in Seg.
On Charades-STA and ActivityNet Captions, the positional prior and the MBR answer, the baselines of \cref{tab:methods}, come from the main-paper run.
\textbf{Bold} marks least watch duration among region types with Cal. at least 0.95.}
\label{tab:supp:watch}
\hypertarget{table.caption.72}{}%
\centering
\scriptsize
\setlength{\tabcolsep}{3.0pt}
\renewcommand{\arraystretch}{0.88}
\begin{adjustbox}{max width=\textwidth}
\begin{tabular}{@{}lll cccc cccc@{}}
\toprule
& & & \multicolumn{4}{c}{IoU\,$\ge$\,0.5 for 80\%} & \multicolumn{4}{c}{IoU\,$\ge$\,0.7 for 80\%} \\
\cmidrule(lr){4-7}\cmidrule(lr){8-11}
\textbf{Benchmark} & \textbf{Model} & \textbf{Method} & Cal. & Hit & Watch$\downarrow$ & Seg. & Cal. & Hit & Watch$\downarrow$ & Seg. \\
\midrule
Charades-STA & Qwen3-VL-4B & Positional prior, no model & \cmark & 0.81 & 0.75 & 1.99 & \cmark & 0.81 & 0.87 & 1.27 \\
 &  & MBR answer at $\tau$, calibrated scale & \cmark & 0.80 & 0.32 & 1.00 & \cmark & 0.82 & 0.45 & 1.00 \\
 &  & Per-second threshold & \cmark & 0.80 & \best{0.31} & 1.07 & \cmark & 0.80 & \best{0.40} & 1.12 \\
 &  & Enumerate-and-cover order & \cmark & 0.80 & 0.33 & 1.14 & \cmark & 0.80 & 0.44 & 1.11 \\
 &  & Gain-per-second anchor & \cmark & 0.80 & 0.38 & 1.23 & \cmark & 0.80 & 0.42 & 1.19 \\
 &  & Exact anchor (main paper) & \cmark & 0.80 & 0.34 & 1.24 & \cmark & 0.80 & 0.43 & 1.13 \\
 &  & Exact anchor with continuation & \cmark & 0.80 & 0.34 & 1.24 & \cmark & 0.80 & 0.43 & 1.13 \\
\cmidrule(lr){2-11}
 & TimeLens2-8B & Positional prior, no model & \cmark & 0.81 & 0.75 & 1.99 & \cmark & 0.81 & 0.87 & 1.27 \\
 &  & MBR answer at $\tau$, calibrated scale & \cmark & 0.81 & 0.33 & 1.00 & \cmark & 0.81 & 0.44 & 1.00 \\
 &  & Per-second threshold & \cmark & 0.80 & \best{0.35} & 1.01 & \cmark & 0.80 & \best{0.46} & 1.01 \\
 &  & Enumerate-and-cover order & \cmark & 0.80 & 0.37 & 1.01 & \cmark & 0.80 & 0.49 & 1.01 \\
 &  & Gain-per-second anchor & \cmark & 0.80 & 0.39 & 1.05 & \cmark & 0.80 & \best{0.46} & 1.02 \\
 &  & Exact anchor (main paper) & \cmark & 0.80 & 0.38 & 1.06 & \cmark & 0.80 & 0.47 & 1.01 \\
 &  & Exact anchor with continuation & \cmark & 0.80 & 0.37 & 1.08 & \cmark & 0.80 & 0.47 & 1.01 \\
\cmidrule(lr){2-11}
 & Qwen3-VL-8B & Positional prior, no model & \cmark & 0.81 & 0.75 & 1.99 & \cmark & 0.81 & 0.87 & 1.27 \\
 &  & MBR answer at $\tau$, calibrated scale & \cmark & 0.81 & 0.32 & 1.00 & \cmark & 0.81 & 0.41 & 1.00 \\
 &  & Per-second threshold & \cmark & 0.80 & \best{0.30} & 1.03 & \cmark & 0.80 & \best{0.40} & 1.07 \\
 &  & Enumerate-and-cover order & \cmark & 0.80 & 0.31 & 1.07 & \cmark & 0.80 & 0.43 & 1.06 \\
 &  & Gain-per-second anchor & \cmark & 0.80 & 0.34 & 1.19 & \cmark & 0.80 & 0.43 & 1.14 \\
 &  & Exact anchor (main paper) & \cmark & 0.80 & 0.31 & 1.13 & \cmark & 0.80 & 0.42 & 1.09 \\
 &  & Exact anchor with continuation & \cmark & 0.80 & 0.31 & 1.13 & \cmark & 0.80 & 0.42 & 1.09 \\
\midrule
QVHighlights & Qwen3-VL-4B & Per-second threshold & \cmark & 0.81 & 0.30 & 1.05 & \cmark & 0.81 & 0.34 & 1.08 \\
 &  & Enumerate-and-cover order & \cmark & 0.80 & \best{0.23} & 1.10 & \cmark & 0.81 & \best{0.31} & 1.12 \\
 &  & Gain-per-second anchor & \cmark & 0.80 & 0.24 & 1.35 & \cmark & 0.81 & 0.32 & 1.24 \\
 &  & Exact anchor (main paper) & \cmark & 0.81 & 0.24 & 1.28 & \cmark & 0.81 & 0.32 & 1.18 \\
 &  & Exact anchor with continuation & \cmark & 0.81 & 0.24 & 1.28 & \cmark & 0.81 & 0.32 & 1.18 \\
\cmidrule(lr){2-11}
 & TimeLens2-8B & Per-second threshold & \cmark & 0.81 & 0.24 & 0.97 & \cmark & 0.81 & 0.28 & 1.00 \\
 &  & Enumerate-and-cover order & \cmark & 0.91 & 0.25 & 1.00 & \cmark & 0.84 & 0.27 & 1.00 \\
 &  & Gain-per-second anchor & \cmark & 0.81 & \best{0.18} & 1.02 & \cmark & 0.81 & 0.27 & 1.04 \\
 &  & Exact anchor (main paper) & \cmark & 0.81 & 0.19 & 1.03 & \cmark & 0.81 & \best{0.25} & 1.02 \\
 &  & Exact anchor with continuation & \cmark & 0.81 & 0.19 & 1.03 & \cmark & 0.81 & \best{0.25} & 1.02 \\
\cmidrule(lr){2-11}
 & Qwen3-VL-8B & Per-second threshold & \cmark & 0.81 & 0.27 & 1.04 & \cmark & 0.81 & 0.30 & 1.10 \\
 &  & Enumerate-and-cover order & \cmark & 0.82 & \best{0.22} & 1.04 & \cmark & 0.81 & \best{0.29} & 1.13 \\
 &  & Gain-per-second anchor & \cmark & 0.81 & 0.25 & 1.35 & \cmark & 0.81 & 0.30 & 1.35 \\
 &  & Exact anchor (main paper) & \cmark & 0.80 & 0.23 & 1.27 & \cmark & 0.80 & 0.31 & 1.26 \\
 &  & Exact anchor with continuation & \cmark & 0.80 & 0.23 & 1.27 & \cmark & 0.80 & 0.31 & 1.26 \\
\midrule
ActivityNet Captions & Qwen3-VL-4B & Positional prior, no model & \cmark & 0.81 & 0.84 & 1.60 & \cmark & 0.81 & 0.89 & 1.01 \\
 &  & MBR answer at $\tau$, calibrated scale & \cmark & 0.82 & 0.56 & 1.00 & \cmark & 0.83 & 0.65 & 1.00 \\
 &  & Per-second threshold & \cmark & 0.80 & 0.51 & 1.12 & \cmark & 0.81 & 0.59 & 1.13 \\
 &  & Enumerate-and-cover order & \cmark & 0.80 & \best{0.47} & 1.15 & \cmark & 0.80 & \best{0.56} & 1.11 \\
 &  & Gain-per-second anchor & \cmark & 0.80 & 0.49 & 1.33 & \cmark & 0.80 & 0.57 & 1.16 \\
 &  & Exact anchor (main paper) & \cmark & 0.80 & 0.49 & 1.36 & \cmark & 0.80 & 0.58 & 1.15 \\
 &  & Exact anchor with continuation & \cmark & 0.80 & 0.48 & 1.45 & \cmark & 0.80 & 0.57 & 1.18 \\
\cmidrule(lr){2-11}
 & TimeLens2-8B & Positional prior, no model & \cmark & 0.81 & 0.84 & 1.60 & \cmark & 0.81 & 0.89 & 1.01 \\
 &  & MBR answer at $\tau$, calibrated scale & \cmark & 0.81 & 0.50 & 1.00 & \cmark & 0.82 & 0.63 & 1.00 \\
 &  & Per-second threshold & \cmark & 0.80 & 0.52 & 1.03 & \cmark & 0.81 & 0.60 & 1.04 \\
 &  & Enumerate-and-cover order & \cmark & 0.80 & \best{0.45} & 1.05 & \cmark & 0.80 & \best{0.58} & 1.03 \\
 &  & Gain-per-second anchor & \cmark & 0.80 & 0.47 & 1.14 & \cmark & 0.80 & 0.60 & 1.05 \\
 &  & Exact anchor (main paper) & \cmark & 0.80 & 0.46 & 1.14 & \cmark & 0.80 & 0.59 & 1.04 \\
 &  & Exact anchor with continuation & \cmark & 0.80 & 0.46 & 1.17 & \cmark & 0.80 & 0.59 & 1.05 \\
\cmidrule(lr){2-11}
 & Qwen3-VL-8B & Positional prior, no model & \cmark & 0.81 & 0.84 & 1.60 & \cmark & 0.81 & 0.89 & 1.01 \\
 &  & MBR answer at $\tau$, calibrated scale & \cmark & 0.82 & 0.53 & 1.00 & \cmark & 0.82 & 0.63 & 1.00 \\
 &  & Per-second threshold & \cmark & 0.80 & 0.46 & 1.10 & \cmark & 0.81 & 0.55 & 1.13 \\
 &  & Enumerate-and-cover order & \cmark & 0.80 & \best{0.44} & 1.15 & \cmark & 0.80 & \best{0.54} & 1.11 \\
 &  & Gain-per-second anchor & \cmark & 0.80 & 0.45 & 1.44 & \cmark & 0.80 & 0.55 & 1.24 \\
 &  & Exact anchor (main paper) & \cmark & 0.80 & 0.45 & 1.42 & \cmark & 0.80 & \best{0.54} & 1.21 \\
 &  & Exact anchor with continuation & \cmark & 0.80 & \best{0.44} & 1.43 & \cmark & 0.80 & \best{0.54} & 1.21 \\
\bottomrule
\end{tabular}
\end{adjustbox}


\end{table*}
